# Supplementary material for: MAIR: A Massive Benchmark for Evaluating Instructed Retrieval
Source: arXiv:2410.10127 source file (2024-10-14)
Supplement: Supplementary file 1 [file appendix.tex]

\section{Data Card}\label{datacard}

\subsection{Academic}

\subsubsection{Competition-Math}
Retrieve solution for mathematical problems. The data is derived from \citet{Hendrycks2021MeasuringCC}, a colleague-level math problem dataset, where we use all solutions in training and test set to compose the corpus.

The following is an example:
\begin{table}[h]\small
\begin{tabularx}{\textwidth}{|>{\itshape}X|}
\hline
\textbf{Instruction} \\\hline
Given a math problem, retrieve a detailed answer to answer this problem.\\\hline
\textbf{Query} \\\hline
Alice and Bob are playing a game. Alice starts first. On Alice's turn, she flips a coin. If she gets a heads, she wins. If not, it becomes Bob's turn. On Bob's turn, he flips a coin. If he gets a tails, he wins. If not, it becomes Alice's turn. What is the probability that Alice wins the game?\\\hline
\textbf{Relevant Document} \\\hline
Alice has a $1/2$ chance of winning the game on her first turn. If she doesn't, then the probability that she wins the game on her second turn is $1/8,$ since she must not win on her first flip ($1/2$ chance), Bob must not win on his first flip ($1/2$ chance), and then Alice must win on her second flip ($1/2$ chance). The probability that she wins the game on her third turn is $1/32,$ and in general, the probability that she wins the game on her 
$k^\text{th}$ turn is $(1/2)^{2k-1}.$
Thus, the probability that Alice wins is an infinite geometric series with first term $1/2$ and common ratio $1/4.$ So, the probability that Alice wins the game is $$\frac{\frac12}{1-\frac14} = \boxed{\frac{2}{3}}.$$ Note that the only difference between the odds of Alice or Bob winning is who goes first. Because Bob goes second, the odds of him winning on his $k^\text{th}$ flip is half of the odds that Alice wins on her $k^\text{th}$ flip, since Alice must first get a tails before Bob gets a chance to win. Thus, if $a$ is Alice's chance of winning, and $b$ is Bob's chance of winning, then $a = 2b.$ Also, since someone must win, $a + b = 1.$ It follows that $a = 2/3$ and $b = 1/3,$ so Alice has a $\boxed{\frac{2}{3}}$ chance of winning the game.
\\\hline
\end{tabularx}
\end{table}

\subsubsection{ProofWiki\_Proof}
\textsc{NaturalProofs}~\citep{Welleck2021NaturalProofsMT} is a multi-domain corpus of mathematical statements and their proofs, written in natural mathematical language. The task is to retrieve proof for a given mathmatical statemnet. ProofWiki\_Proof is \url{https://proofwiki.org/}

The following is an example:
\begin{center}\small
\begin{xltabular}{\textwidth}{|>{\itshape}X|}
\hline
\textbf{Instruction} \\\hline
Given a mathematical statement, retrieve its proofs written in natural mathematical language.\\\hline
\textbf{Query} \\\hline
Intersection of Left Cosets of Subgroups is Left Coset of Intersection
Let $G$ be a [[Definition:Group|group]]. Let $H, K \le G$ be [[Definition:Subgroup|subgroups]] of $G$. Let $a, b \in G$. Let: :$a H \cap b K \ne \O$ where $a H$ denotes the [[Definition:Left Coset|left coset]] of $H$ by $a$. Then $a H \cap b K$ is a [[Definition:Left Coset|left coset]] of $H \cap K$.\\\hline
\textbf{Relevant Document} \\\hline
Let $x \in aH \cap bK$. Then: \\
        \begin{equation}
            \begin{aligned}
                x &\in aH \\
                \Rightarrow xH &= aH & \text{(Left Cosets are Equal iff Element in Other Left Coset)}
            \end{aligned}
        \end{equation} \\
        and similarly: \\
        \begin{equation}
            \begin{aligned}
                x &\in bK \\
                \Rightarrow xK &= bK & \text{(Left Cosets are Equal iff Element in Other Left Coset)}
            \end{aligned}
        \end{equation} \\
        Hence: \\
        \begin{equation}
            \begin{aligned}
                aH \cap bK &= xH \cap xK \\
                           &= x (H \cap K) & \text{(Corollary to Product of Subset with Intersection)}
            \end{aligned}
        \end{equation} \\
        Hence the result by definition of left coset. \\
        \(\blacksquare\)
\\\hline
\end{xltabular}
\end{center}

\subsubsection{Stacks\_Proof}
The Stacks domain of from \textsc{NaturalProofs}.

\begin{center}\small
\begin{xltabular}{\textwidth}{|>{\itshape}X|}
\hline
\textbf{Instruction} \\\hline
Given a mathematical statement, retrieve its proofs written in natural mathematical language.\\\hline
\textbf{Query} \\\hline
stacks-cohomology-lemma-quasi-coherent-weak-serre

Let $\mathcal{X}$ be an algebraic stack.
\begin{enumerate}
    \item $\QCoh(\mathcal{O}_{\mathcal{X}_{lisse,\etale}})$ is a weak Serre subcategory of $\textit{Mod}(\mathcal{O}_{\mathcal{X}_{lisse,\etale}})$.
    \item $\QCoh(\mathcal{O}_{\mathcal{X}_{flat,fppf}})$ is a weak Serre subcategory of $\textit{Mod}(\mathcal{O}_{\mathcal{X}_{flat,fppf}})$.
\end{enumerate}
\\\hline
\textbf{Relevant Document} \\\hline
We will verify conditions (1), (2), (3), (4) of Homology, Lemma "homology-lemma-characterize-weak-serre-subcategory". Since $0$ is a quasi-coherent module on any ringed site we see that (1) holds. By definition $\QCoh(\mathcal{O})$ is a strictly full subcategory $\textit{Mod}(\mathcal{O})$, so (2) holds. Let $\varphi : \mathcal{G} \to \mathcal{F}$ be a morphism of quasi-coherent modules on $\mathcal{X}_{lisse,\etale}$ or $\mathcal{X}_{flat,fppf}$. We have $g^*g_!\mathcal{F} = \mathcal{F}$ and similarly for $\mathcal{G}$ and $\varphi$, see Lemma "lemma-lisse-etale-modules". By Lemma "lemma-shriek-quasi-coherent" we see that $g_!\mathcal{F}$ and $g_!\mathcal{G}$ are quasi-coherent $\mathcal{O}_\mathcal{X}$-modules. Hence we see that $\Ker(g_!\varphi)$ and $\Coker(g_!\varphi)$ are quasi-coherent modules on $\mathcal{X}$. Since $g^*$ is exact (see Lemma "lemma-lisse-etale") we see that $g^*\Ker(g_!\varphi) = \Ker(g^*g_!\varphi) = \Ker(\varphi)$ and $g^*\Coker(g_!\varphi) = \Coker(g^*g_!\varphi) = \Coker(\varphi)$ are quasi-coherent too (see Lemma "lemma-quasi-coherent"). This proves (3). \medskip \noindent Finally, suppose that 
\[ 0 \to \mathcal{F} \to \mathcal{E} \to \mathcal{G} \to 0 \] 
is an extension of $\mathcal{O}_{\mathcal{X}_{lisse,\etale}}$-modules (resp.\ $\mathcal{O}_{\mathcal{X}_{flat,fppf}}$-modules) with $\mathcal{F}$ and $\mathcal{G}$ quasi-coherent. We have to show that $\mathcal{E}$ is quasi-coherent on $\mathcal{X}_{lisse,\etale}$ (resp.\ $\mathcal{X}_{flat,fppf}$). We strongly urge the reader to write out what this means on a napkin and prove it him/herself rather than reading the somewhat labyrinthine proof that follows. By Lemma "lemma-quasi-coherent" this is true if and only if $g_!\mathcal{E}$ is quasi-coherent. By Lemmas "lemma-check-qc-on-etale-covering" and "lemma-lisse-etale-functorial" we may check this after replacing $\mathcal{X}$ by a smooth (resp.\ fppf) cover. Choose a scheme $U$ and a smooth surjective morphism $U \to \mathcal{X}$. By definition there exists an \'etale (resp.\ fppf) covering $\{U_i \to U\}_i$ such that $\mathcal{G}$ has a global presentation over each $U_i$. Replacing $\mathcal{X}$ by $U_i$ (which is permissible by the discussion above) we may assume that the site $\mathcal{X}_{lisse,\etale}$ (resp.\ $\mathcal{X}_{flat,fppf}$) has a final object $U$ (in other words $\mathcal{X}$ is representable by the scheme $U$) and that $\mathcal{G}$ has a global presentation 
\[ \bigoplus\nolimits_{j \in J} \mathcal{O} \longrightarrow \bigoplus\nolimits_{i \in I} \mathcal{O} \longrightarrow \mathcal{G} \longrightarrow 0 \] 
of $\mathcal{O}$-modules where $\mathcal{O} = \mathcal{O}_{\mathcal{X}_{lisse,\etale}}$ (resp.\ $\mathcal{O} = \mathcal{O}_{\mathcal{X}_{flat,fppf}}$). Let $\mathcal{E}'$ be the pullback of $\mathcal{E}$ via the map $\bigoplus\nolimits_{i \in I} \mathcal{O} \to \mathcal{G}$. Then we see that $\mathcal{E}$ is the cokernel of a map $\bigoplus\nolimits_{j \in J} \mathcal{O} \to \mathcal{E}'$ hence by property (3) which we proved above, it suffices to prove that $\mathcal{E}'$ is quasi-coherent.
\colorbox{mediumgray}{\textup{[...]}}
\\\hline
\end{xltabular}
\end{center}

\subsubsection{Stein\_Proof}

\begin{center}\small
\begin{xltabular}{\textwidth}{|>{\itshape}X|}
\hline
\textbf{Instruction} \\\hline
Given a mathematical statement, retrieve its proofs written in natural mathematical language.\\\hline
\textbf{Query} \\\hline
Fundamental Theorem of Arithmetic: Every natural number can be written as a product of primes uniquely up to order.
\\\hline
\textbf{Relevant Document} \\\hline
We only prove that $\gcd(a,b) = \gcd(a,b-a)$, since the other cases are proved in a similar way. Suppose $d\mid a$ and $d\mid b$, so there exist integers $c_1$ and $c_2$ such that $dc_1 = a$ and $dc_2 = b$. Then $b - a = dc_2 - dc_1 = d(c_2-c_1)$, so $d\mid b-a$. Thus $\gcd(a,b)\leq \gcd(a,b-a)$, since the set over which we are taking the max for $\gcd(a,b)$ is a subset of the set for $\gcd(a,b-a)$. The same argument with $a$ replaced by $-a$ and $b$ replaced by $b-a$, shows that $\gcd(a,b-a)=\gcd(-a,b-a)\leq \gcd(-a,b)=\gcd(a,b)$, which proves that $\gcd(a,b)=\gcd(a,b-a)$. 
\\\hline
\end{xltabular}
\end{center}

\subsubsection{Trench\_Proof}
\begin{center}\small
\begin{xltabular}{\textwidth}{|>{\itshape}X|}
\hline
\textbf{Instruction} \\\hline
Given a mathematical statement, retrieve its proofs written in natural mathematical language.\\\hline
\textbf{Query} \\\hline
If $a$ and $b$ are any two real numbers, then 
\begin{equation} \label{eq:1.1.4} 
|a-b|\ge\big||a|-|b|\big| 
\end{equation} 
and 
\begin{equation} \label{eq:1.1.5} 
|a+b|\ge\big||a|-|b|\big|. 
\end{equation}
\\\hline
\textbf{Relevant Document} \\\hline
Replacing $a$ by $a-b$ in [Ref] yields
\[ |a| \le |a-b| + |b|, \]
so
\begin{equation} \label{eq:1.1.6}
|a-b| \ge |a| - |b|.
\end{equation}
Interchanging $a$ and $b$ here yields
\[ |b-a| \ge |b| - |a|, \]
which is equivalent to
\begin{equation} \label{eq:1.1.7}
|a-b| \ge |b| - |a|,
\end{equation}
since $|b-a| = |a-b|$. Since
\[ \big||a| - |b|\big| = \begin{cases}
|a| - |b| & \text{if } |a| > |b|,\\
|b| - |a| & \text{if } |b| > |a|,
\end{cases} \]
\eqref{eq:1.1.6} and \eqref{eq:1.1.7} imply \eqref{eq:1.1.4}. Replacing $b$ by $-b$ in \eqref{eq:1.1.4} yields \eqref{eq:1.1.5}, since $|-b| = |b|$.
\\\hline
\end{xltabular}
\end{center}

\subsubsection{ProofWiki\_Reference}

\begin{center}\small
\begin{xltabular}{\textwidth}{|>{\itshape}X|}
\hline
\textbf{Instruction} \\\hline
Given a mathematical claim, retrieve the set of references (theorems, lemmas, definitions) that occur in its proof.\\\hline
\textbf{Query} \\\hline
Kernel of Group Action is Normal Subgroup \\
Let $G$ be a \emph{group} whose \emph{identity} is $e$. Let $X$ be a \emph{set}. Let $\phi: G \times X \to X$ be a \emph{group action}. Let $G_0$ denote the \emph{kernel of $\phi$}. Then $G_0$ is a \emph{normal subgroup} of $G$.
\\\hline
\textbf{Relevant Document} \\\hline
Stabilizer is Subgroup \\
Let $\struct{G, \circ}$ be a \textbf{group} which \textbf{acts on} a \textbf{set} $X$. Let $\Stab(x)$ be the \textbf{stabilizer of $x$ by $G$}. Then for each $x \in X$, $\Stab(x)$ is a \textbf{subgroup} of $G$.
\\\hline
\end{xltabular}
\end{center}

\subsubsection{Stacks\_Reference}

\begin{center}\small
\begin{xltabular}{\textwidth}{|>{\itshape}X|}
\hline
\textbf{Instruction} \\\hline
Given a mathematical claim, retrieve the set of references (theorems, lemmas, definitions) that occur in its proof.
\\\hline
\textbf{Query} \\\hline
stacks-cohomology-lemma-relative-leray
Let $f : \mathcal{X} \to \mathcal{Y}$ and $g : \mathcal{Y} \to \mathcal{Z}$ be quasi-compact and quasi-separated morphisms of algebraic stacks. Let $\mathcal{F}$ be a quasi-coherent sheaf on $\mathcal{X}$. Then there exists a spectral sequence with $E_2$-page
\[ E_2^{p, q} = R^p g_{\text{QCoh}, *} (R^q f_{\text{QCoh}, *} \mathcal{F}) \]
converging to $R^{p+q} (g \circ f)_{\text{QCoh}, *} \mathcal{F}$.
\\\hline
\textbf{Relevant Document} \\\hline
sites-cohomology-lemma-relative-Leray \\
Let $f : (\Sh(\mathcal{C}), \mathcal{O}_\mathcal{C}) \to (\Sh(\mathcal{D}), \mathcal{O}_\mathcal{D})$ and $g : (\Sh(\mathcal{D}), \mathcal{O}_\mathcal{D}) \to (\Sh(\mathcal{E}), \mathcal{O}_\mathcal{E})$ be morphisms of ringed topoi. Let $\mathcal{F}$ be an $\mathcal{O}_\mathcal{C}$-module. There is a spectral sequence with 
\[ E_2^{p, q} = R^p g_*(R^q f_* \mathcal{F}) \]
converging to $R^{p + q}(g \circ f)_* \mathcal{F}$. This spectral sequence is functorial in $\mathcal{F}$, and there is a version for bounded below complexes of $\mathcal{O}_\mathcal{C}$-modules.
\\\hline
\end{xltabular}
\end{center}

\subsubsection{Stein\_Reference}

\begin{center}\small
\begin{xltabular}{\textwidth}{|>{\itshape}X|}
\hline
\textbf{Instruction} \\\hline
Given a mathematical claim, retrieve the set of references (theorems, lemmas, definitions) that occur in its proof.
\\\hline
\textbf{Query} \\\hline
Euclid\\
Let~$p$ be a prime and $a, b\in \mathbb{N}$. If $p \mid ab$ then $p \mid a$ or $p \mid b$.
\\\hline
\textbf{Relevant Document} \\\hline
For any integers $a,b,n$, we have $\gcd(an,bn) = \gcd(a,b)\cdot |n|$.
\\\hline
\end{xltabular}
\end{center}

\subsubsection{Trench\_Reference}
\begin{center}\small
\begin{xltabular}{\textwidth}{|>{\itshape}X|}
\hline
\textbf{Instruction} \\\hline
Given a mathematical claim, retrieve the set of references (theorems, lemmas, definitions) that occur in its proof.
\\\hline
\textbf{Query} \\\hline
The set of irrational numbers is dense in the reals; that is, if $a$ and $b$ are real numbers with $a<b$, there is an irrational number $t$ such that $a<t<b$.
\\\hline
\textbf{Relevant Document} \\\hline
The rational numbers are dense in the reals; that is, if $a$ and $b$ are real numbers with $a<b$, there is a rational number $\frac{p}{q}$ such that $a < \frac{p}{q} < b$.
\\\hline
\end{xltabular}
\end{center}

\subsubsection{TAD}

\begin{center}\small
\begin{xltabular}{\textwidth}{|>{\itshape}X|}
\hline
\textbf{Instruction} \\\hline
Given a paragraph from the related work section of a paper, where citations are masked with the symbol '\&', retrieve the abstracts of the cited reference papers.
\\\hline
\textbf{Query} \\\hline
in \& and \& , the authors of \& abandon the quantization of image regions . with the same conditional independence assumptions than in their previous model \& , the continuous image region representation , modeled by a gaussian mixture model ( gmm ) , improves the image annotation performance . an additional modification is proposed in \& , where a multiple bernoulli distribution for image captions replaces the multinomial distribution.
\\\hline
\textbf{Relevant Document} \\\hline
despite pre-trained language models have proven useful for learning high-quality semantic representations , these models are still vulnerable to simple perturbations . recent works aimed to improve the robustness of pre-trained models mainly focus on adversarial training from perturbed examples with similar semantics , neglecting the utilization of different or even opposite semantics . different from the image processing field , the text is discrete and few word substitutions can cause significant semantic changes . to study the impact of semantics caused by small perturbations , we conduct a series of pilot experiments and surprisingly find that adversarial training is useless or even harmful for the model to detect these semantic changes . to address this problem , we propose contrastive learning with semantic negative examples ( cline ) , which constructs semantic negative examples unsupervised to improve the robustness under semantically adversarial attacking . by comparing with similar and opposite semantic examples , the model can effectively perceive the semantic changes caused by small perturbations . empirical results show that our approach yields substantial improvements on a range of sentiment analysis , reasoning , and reading comprehension tasks . and cline also ensures the compactness within the same semantics and separability across different semantics in sentence-level .
\\\hline
\end{xltabular}
\end{center}

\subsubsection{TAS2}

\begin{center}\small
\begin{xltabular}{\textwidth}{|>{\itshape}X|}
\hline
\textbf{Instruction} \\\hline
Given a paragraph from the related work section of a paper, where citations are masked with the symbol '\&', retrieve the abstracts of the cited reference papers.
\\\hline
\textbf{Query} \\\hline
extracting summaryworthy sentences from the source documents is important even if the ultimate goal is to generate abstracts . recent abstractive studies recognize the importance of separating salience estimation from text generation so as to reduce the amount of training data required by encoderdecoder models \& \& \& . an extractive method is often leveraged to identify salient source sentences , then a neural text generator rewrites the selected sentences into an abstract . our pursuit of the dpp method is especially meaningful in this context . as described in the next section , dpp has an extraordinary ability to distinguish redundant descriptions , thereby avoiding passing redundant content to the abstractor that can cause an encoderdecoder model to fail .
\\\hline
\textbf{Relevant Document} \\\hline
neural network-based methods for abstractive summarization produce outputs that are more fluent than other techniques , but perform poorly at content selection . this work proposes a simple technique for addressing this issue use a data-efficient content selector to over-determine phrases in a source document that should be part of the summary . we use this selector as a bottom-up attention step to constrain the model to likely phrases . we show that this approach improves the ability to compress text , while still generating fluent summaries . this two-step process is both simpler and higher performing than other end-toend content selection models , leading to significant improvements on rouge for both the cnn-dm and nyt corpus . furthermore , the content selector can be trained with as little as 1,000 sentences , making it easy to transfer a trained summarizer to a new domain .
\\\hline
\end{xltabular}
\end{center}

\subsubsection{StackMathQA}

\begin{center}\small
\begin{xltabular}{\textwidth}{|>{\itshape}X|}
\hline
\textbf{Instruction} \\\hline
Given a math question, retrieve its answers from various Stack Exchange sites.
\\\hline
\textbf{Query} \\\hline
Help with convergence in distribution $Y$ is a random variable with $M(t) = \frac{1}{(2-\exp(t))^s}$. Does $\frac{Y-E(Y)}{\sqrt{\operatorname{Var}(Y)}}$ converge in distribution as $s$ tends to infinity? I let $Z = \frac{Y-E(Y)}{\sqrt{\operatorname{Var}(Y)}}$. Differentiating the MGF of $Y$ and letting $t = 0$ we have $E(Y) = s$,
$E(Y^2) = s^2 + 2s$,
$\operatorname{Var}(Y) = 2s$. Thus MGF of $Z$:
\[
E(\exp(tz)) = E\left(\exp\left(\frac{t(y-s)}{\sqrt{2s}}\right)\right)
= E\left(\exp\left(\frac{ty}{\sqrt{2s}}\right)\exp\left(\frac{-ts}{\sqrt{2s}}\right)\right)
= \exp\left(\frac{-ts}{\sqrt{2s}}\right)\frac{1}{\left(2-\exp\left(\frac{t}{\sqrt{2s}}\right)\right)^s}.
\]
\\\hline
\textbf{Relevant Document} \\\hline
As you have determined:
\[
M_Z(t) = \mathbb{E}(\exp(t Z)) = \frac{\exp\left(-t \frac{s}{\sqrt{2s}}\right)}{\left( 2 - \exp\left(\frac{t}{\sqrt{2s}} \right) \right)^s} = \left( \frac{\exp\left(-t \frac{1}{\sqrt{2s}}\right)}{ 2 - \exp\left(\frac{t}{\sqrt{2s}} \right) } \right)^s
\]
In order to determine large $s$ behavior, use Taylor series:
\[
\frac{\exp\left(-t \frac{1}{\sqrt{2s}}\right)}{ 2 - \exp\left(\frac{t}{\sqrt{2s}} \right) } = \frac{1- \frac{t}{\sqrt{2s}} + \frac{t^2}{4 s} + o\left(\frac{t^2}{s}\right)}{ 1- \frac{t}{\sqrt{2s}} - \frac{t^2}{4 s} + o\left(\frac{t^2}{s}\right) } = 1 + \frac{t^2}{2s} + o\left(\frac{t^2}{s}\right)
\]
Thus 
\[
M_Z(t) = \left( 1 + \frac{t^2}{2s} + o\left(\frac{t^2}{s}\right) \right)^s
\]
The large $s$ limit is now easy to find:
\[
\lim_{s \to \infty} M_Z(t) = \exp\left( \frac{t^2}{2} \right)
\]
This is the mgf of the standard normal variable, as expected by CLT.
\\\hline
\end{xltabular}
\end{center}

\subsubsection{SciDocs}

\begin{center}\small
\begin{xltabular}{\textwidth}{|>{\itshape}X|}
\hline
\textbf{Instruction} \\\hline
Given a scientific paper title, retrieve paper abstracts that are cited by the given paper.
\\\hline
\textbf{Query} \\\hline
On Parallelizing the Multiprocessor Scheduling Problem
\\\hline
\textbf{Relevant Document} \\\hline
Hypertool: A Programming Aid for Message-Passing Systems | As both the number of processors and the complexity of problems to be solved increase, programming multiprocessing systems becomes more di cult and errorprone. This paper discusses programming assistance and automation concepts and their application to a program development tool for message-passing systems called Hypertool. It performs scheduling and handles the communication primitive insertion automatically. Two algorithms, based on the critical-path method, are presented for scheduling processes statically. Hypertool also generates the performance estimates and other program quality measures to help programmers in improving their algorithms and programs.
\\\hline
\end{xltabular}
\end{center}

\subsubsection{SciFact}

\begin{center}\small
\begin{xltabular}{\textwidth}{|>{\itshape}X|}
\hline
\textbf{Instruction} \\\hline
Given a scientific claim, retrieve documents that support or refute the claim.
\\\hline
\textbf{Query} \\\hline
0-dimensional biomaterials show inductive properties.
\\\hline
\textbf{Relevant Document} \\\hline
New opportunities: the use of nanotechnologies to manipulate and track stem cells.Nanotechnologies are emerging platforms that could be useful in measuring, understanding, and manipulating stem cells. Examples include magnetic nanoparticles and quantum dots for stem cell labeling and in vivo tracking; nanoparticles, carbon nanotubes, and polyplexes for the intracellular delivery of genes/oligonucleotides and protein/peptides; and engineered nanometer-scale scaffolds for stem cell differentiation and transplantation. This review examines the use of nanotechnologies for stem cell tracking, differentiation, and transplantation. We further discuss their utility and the potential concerns regarding their cytotoxicity.
\\\hline
\end{xltabular}
\end{center}

\subsubsection{FairRanking-2020}

\begin{center}\small
\begin{xltabular}{\textwidth}{|>{\itshape}X|}
\hline
\textbf{Instruction} \\\hline
Given a query, retrieve relevant academic articles. Ensure provide fair exposure to different groups of authors, where the group definitions could based on demographics, stature, topic, and others.
\\\hline
\textbf{Query} \\\hline
hemophilia
\\\hline
\textbf{Relevant Document} \\\hline
Bleeding in carriers of hemophilia. \newline

A wide range of factor VIII and IX levels is observed in heterozygous carriers of hemophilia as well as in noncarriers. In female carriers, extreme lyonization may lead to low clotting factor levels. We studied the effect of heterozygous hemophilia carriership on the occurrence of bleeding symptoms. A postal survey was performed among most of the women who were tested for carriership of hemophilia in the Netherlands before 2001. The questionnaire included items on personal characteristics, characteristics of hemophilia in the affected family members, and carrier testing and history of bleeding problems such as bleeding after tooth extraction, bleeding after tonsillectomy, and other operations. Information on clotting factor levels was obtained from the hospital charts. Logistic regression was used to assess the relation of carrier status and clotting factor levels with the occurrence of hemorrhagic events. In 2004, 766 questionnaires were sent, and 546 women responded (80\%). Of these, 274 were carriers of hemophilia A or B. The median clotting factor level of carriers was 0.60 IU/mL (range, 0.05-2.19 IU/mL) compared with 1.02 IU/mL (range, 0.45-3.28 IU/mL) in noncarriers. Clotting factor levels from 0.60 to 0.05 IU/mL were increasingly associated with prolonged bleeding from small wounds and prolonged bleeding after tooth extraction, tonsillectomy, and operations. Carriers of hemophilia bleed more than other women, especially after medical interventions. Our findings suggest that not only clotting factor levels at the extreme of the distribution, resembling mild hemophilia, but also mildly reduced clotting factor levels between 0.41 and 0.60 IU/mL are associated with bleeding. \newline

Year=2006.0 \newline
Venue=Blood \newline
Citations=103.0 \newline
Key Citations=\\\hline
\end{xltabular}
\end{center}

\subsection{Code}

\subsubsection{APPS}

\begin{center}\small
\begin{xltabular}{\textwidth}{|>{\itshape}X|}
\hline
\textbf{Instruction} \\\hline
Given a programming problem, retrieve Python solutions that solve this problem.
\\\hline
\textbf{Query} \\\hline
You are given a string $s$. You have to reverse it — that is, the first letter should become equal to the last letter before the reversal, the second letter should become equal to the second-to-last letter before the reversal — and so on. For example, if your goal is to reverse the string "abddea", you should get the string "aeddba". To accomplish your goal, you can swap the neighboring elements of the string.

Your task is to calculate the minimum number of swaps you have to perform to reverse the given string.

-----Input-----

The first line contains one integer $n$ ($2 \le n \le 200,000$) — the length of $s$.

The second line contains $s$ — a string consisting of $n$ lowercase Latin letters.

-----Output-----

Print one integer — the minimum number of swaps of neighboring elements you have to perform to reverse the string.

-----Examples-----

Input

5
aaaza

Output

2\\
\colorbox{mediumgray}{\textup{[...]}}
\\\hline
\textbf{Relevant Document} \\\hline
\texttt{class BIT():\newline
\hspace*{0.5cm} def \_\_init\_\_(self,n):\newline
\hspace*{1cm} self.BIT=[0]*(n+1)\newline
\hspace*{1cm} self.num=n\newline
\newline
\hspace*{0.5cm} def query(self,idx):\newline
\hspace*{1cm} res\_sum = 0\newline
\hspace*{1cm} while idx > 0:\newline
\hspace*{1.5cm} res\_sum += self.BIT[idx]\newline
\hspace*{1.5cm} idx -= idx\&(-idx)\newline
\hspace*{1cm} return res\_sum\newline
\newline
\hspace*{0.5cm} \#Ai += x O(logN)\newline
\hspace*{0.5cm} def update(self,idx,x):\newline
\hspace*{1cm} while idx <= self.num:\newline
\hspace*{1.5cm} self.BIT[idx] += x\newline
\hspace*{1.5cm} idx += idx\&(-idx)\newline
\hspace*{1cm} return\newline}
\colorbox{mediumgray}{\textup{[...]}}
\\\hline
\end{xltabular}
\end{center}

\subsubsection{CodeEditSearch}

\begin{center}\small
\begin{xltabular}{\textwidth}{|>{\itshape}X|}
\hline
\textbf{Instruction} \\\hline
Given a GitHub commit message, retrieve the relevant code diff files associated with this commit and implement the changes described.
\\\hline
\textbf{Query} \\\hline
Add comparison to "real" value.
\\\hline
\textbf{Relevant Document} \\\hline
\texttt{\hspace*{0mm}--- \newline
\hspace*{0mm}+++ \newline
\hspace*{0mm}@@ -1,6 +1,9 @@ \newline
\hspace*{0mm}/** @file.cc \newline
\hspace*{3mm}* pi approximation \newline
\hspace*{3mm}*/ \newline
\hspace*{0mm}+ \newline
\hspace*{0mm}+\#include <cmath> \newline
\hspace*{0mm}+\#include <iomanip> \newline
\hspace*{0mm}\#include <iostream> \newline
\hspace*{0mm}\#include <random> \newline
\hspace*{0mm} \newline
\hspace*{0mm}@@ -29,5 +32,8 @@ \newline
\hspace*{3mm}int main(int argc, char *argv[])  \newline
\hspace*{6mm}std::random\_device rd; \newline
\hspace*{6mm}std::mt19937 rng(rd()); \newline
\hspace*{6mm}-  std::cout << "pi = " << ApproximatePi(10000000, rng) << std::endl; \newline
\hspace*{6mm}+  double pi = ApproximatePi(10000000, rng); \newline
\hspace*{6mm}+  std::cout << std::setprecision(20) \newline
\hspace*{6mm}+            << "    pi = " << pi << std::endl \newline
\hspace*{6mm}+            << "pi - pi = " << pi - M\_PI << std::endl;}
\\\hline
\end{xltabular}
\end{center}

\subsubsection{CodeSearchNet}

\begin{center}\small
\begin{xltabular}{\textwidth}{|>{\itshape}X|}
\hline
\textbf{Instruction} \\\hline
Given the documentation string for a function, retrieve the corresponding function's code.
\\\hline
\textbf{Query} \\\hline
Returns the link to the checkout page on this site

@param boolean urlSegment If set to TRUE, only returns the URLSegment field

@return string Link to checkout page
\\\hline
\textbf{Relevant Document} \\\hline
\texttt{public static function find\_link(\$urlSegment = false, \$action = false, \$id = false) \{ \newline
    \hspace*{0.5cm} \$base = CartPageController::config()->url\_segment; \newline
    \hspace*{0.5cm} if (\$page = self::get()->first()) \{ \newline
    \hspace*{1cm} \$base = \$page->Link(); \newline
    \hspace*{0.5cm} \} \newline
    \hspace*{0.5cm} return Controller::join\_links(\$base, \$action, \$id); \newline
  \} }
\\\hline
\end{xltabular}
\end{center}

\subsubsection{Conala}

\begin{center}\small
\begin{xltabular}{\textwidth}{|>{\itshape}X|}
\hline
\textbf{Instruction} \\\hline
Given a natural language intent (e.g., a StackOverflow question), retrieve relevant documents from Python libraries on DevDocs that help address the intent. The documents should contain descriptions of single Python functions.
\\\hline
\textbf{Query} \\\hline
get value of the environment variable 'KEY\_THAT\_MIGHT\_EXIST' with default value `default\_value`
\\\hline
\textbf{Relevant Document} \\\hline
python.library.os\#os.getenv\newline
os.getenv(key, default=None)\newline
Return the value of the environment variable key if it exists, or default if it doesn't. key, default and the result are str. On Unix, keys and values are decoded with sys.getfilesystemencoding() and 'surrogateescape' error handler. Use os.getenvb() if you would like to use a different encoding. Availability: most flavors of Unix, Windows.
\\\hline
\end{xltabular}
\end{center}

\subsubsection{TLDR}

\begin{center}\small
\begin{xltabular}{\textwidth}{|>{\itshape}X|}
\hline
\textbf{Instruction} \\\hline
Given a natural language intent for Bash commands, retrieve relevant Bash manual documents that describe a single concept, such as an argument flag, to address the intent.
\\\hline
\textbf{Query} \\\hline
delete an ipc queue by key
\\\hline
\textbf{Relevant Document} \\\hline
ipcrm removes System V inter-process communication (IPC) objects and associated data structures from the system. In order to delete such objects, you must be superuser, or the creator or owner of the object.
\\\hline
\end{xltabular}
\end{center}

\subsubsection{HumanEval-X}

\begin{center}\small
\begin{xltabular}{\textwidth}{|>{\itshape}X|}
\hline
\textbf{Instruction} \\\hline
Given a function declaration and its accompanying docstring, retrieve the subsequent code of the function.
\\\hline
\textbf{Query} \\\hline
\texttt{import (} \newline
  \hspace*{2em} \texttt{"math"} \newline
  \hspace*{2em} \texttt{"strconv"} \newline
  \hspace*{2em} \texttt{"strings"} \newline
  \texttt{)} \newline
  \newline
  \texttt{// Create a function that takes a value (string) representing a number} \newline
  \texttt{// and returns the closest integer to it. If the number is equidistant} \newline
  \texttt{// from two integers, round it away from zero.} \newline
  \texttt{// Examples} \newline
\colorbox{mediumgray}{\textup{[...]}}\newline
  \texttt{// Note:} \newline
  \texttt{// Rounding away from zero means that if the given number is equidistant} \newline
  \texttt{// from two integers, the one you should return is the one that is the} \newline
  \texttt{// farthest from zero. For example ClosestInteger("14.5") should} \newline
  \texttt{// return 15 and ClosestInteger("-14.5") should return -15.} \newline
  \texttt{func ClosestInteger(value string) int \{}
\\\hline
\textbf{Relevant Document} \\\hline
\texttt{if strings.Count(value, ".") == 1 \{} \newline
\hspace*{2em} \texttt{// remove trailing zeros} \newline
\hspace*{2em} \texttt{for value[len(value)-1] == '0' \{} \newline
\hspace*{4em} \texttt{value = value[:len(value)-1]} \newline
\hspace*{2em} \texttt{\}} \newline
\texttt{\}} \newline
\texttt{var res float64} \newline
\texttt{num, \_ := strconv.ParseFloat(value, 64)} \newline
\texttt{if len(value) >= 2 \&\& value[len(value)-2:] == ".5" \{} \newline
\hspace*{2em} \texttt{if num > 0 \{} \newline
\hspace*{4em} \texttt{res = math.Ceil(num)} \newline
\hspace*{2em} \texttt{\} else \{} \newline
\hspace*{4em} \texttt{res = math.Floor(num)} \newline
\hspace*{2em} \texttt{\}} \newline
\colorbox{mediumgray}{\textup{[...]}}
\\\hline
\end{xltabular}
\end{center}

\subsubsection{LeetCode}

\begin{center}\small
\begin{xltabular}{\textwidth}{|>{\itshape}X|}
\hline
\textbf{Instruction} \\\hline
Given a LeetCode question, retrieve the solution written in java. Solutions in other programming languages are not relevant.
\\\hline
\textbf{Query} \\\hline
\textbf{Title: Target Sum}

\textbf{Content:} You are given an integer array \texttt{nums} and an integer \texttt{target}.

You want to build an \textbf{expression} out of \texttt{nums} by adding one of the symbols `'+'` and `'-'` before each integer in \texttt{nums} and then concatenate all the integers.

For example, if \texttt{nums = [2, 1]}, you can add a `'+'` before `2` and a `'-'` before `1` and concatenate them to build the expression ``+2-1 ``.

Return the number of different \textbf{expressions} that you can build, which evaluates to \texttt{target}.

\textbf{Example 1:}

\textbf{Input:} nums = \([1,1,1,1,1]\), target = 3

\textbf{Output:} 5

\textbf{Explanation:} There are 5 ways to assign symbols to make the sum of nums be target 3.

-1 + 1 + 1 + 1 + 1 = 3

+1 - 1 + 1 + 1 + 1 = 3

\colorbox{mediumgray}{\textup{[...]}}
\\\hline
\textbf{Relevant Document} \\\hline
\texttt{public int findTargetSumWays(int[] nums, int target) \{} \newline
  \hspace*{2em} \texttt{int sum = 0;} \newline
  \hspace*{2em} \texttt{for (int num : nums) sum += num;} \newline
  \hspace*{2em} \texttt{if (sum < target || (sum + target) \% 2 != 0) return 0;} \newline
  \hspace*{2em} \texttt{int target\_sum = (sum + target) / 2;} \newline
  \hspace*{2em} \texttt{int[] dp = new int[target\_sum + 1];} \newline
  \hspace*{2em} \texttt{dp[0] = 1;} \newline
  \hspace*{2em} \texttt{for (int num : nums) \{} \newline
  \hspace*{4em} \texttt{for (int j = target\_sum; j >= num; j--) \{} \newline
  \hspace*{6em} \texttt{dp[j] += dp[j - num];} \newline
  \hspace*{4em} \texttt{\}} \newline
  \hspace*{2em} \texttt{\}} \newline
  \hspace*{2em} \texttt{return dp[target\_sum];} \newline
  \texttt{\}} \newline
  \newline
  The problem can be reduced to a subset sum problem by doing some simple math. First, calculate the sum of all numbers in the array. If the sum of integers is less than the target value or the total sum with the target value is odd, there are no possible combinations.
\colorbox{mediumgray}{\textup{[...]}}
\\\hline
\end{xltabular}
\end{center}

\subsubsection{MBPP}

\begin{center}\small
\begin{xltabular}{\textwidth}{|>{\itshape}X|}
\hline
\textbf{Instruction} \\\hline
Given a description of a programming task, retrieve a Python solution.
\\\hline
\textbf{Query} \\\hline
Write a python function to find the first non-repeated character in a given string.
\\\hline
\textbf{Relevant Document} \\\hline
\texttt{def first\_non\_repeating\_character(str1):} \newline
  \hspace*{2em} \texttt{char\_order = []} \newline
  \hspace*{2em} \texttt{ctr = \{\}} \newline
  \hspace*{2em} \texttt{for c in str1:} \newline
  \hspace*{4em} \texttt{if c in ctr:} \newline
  \hspace*{6em} \texttt{ctr[c] += 1} \newline
  \hspace*{4em} \texttt{else:} \newline
  \hspace*{6em} \texttt{ctr[c] = 1} \newline
  \hspace*{6em} \texttt{char\_order.append(c)} \newline
  \hspace*{2em} \texttt{for c in char\_order:} \newline
  \hspace*{4em} \texttt{if ctr[c] == 1:} \newline
  \hspace*{6em} \texttt{return c} \newline
  \hspace*{2em} \texttt{return None}
\\\hline
\end{xltabular}
\end{center}

\subsubsection{RepoBench}

\begin{center}\small
\begin{xltabular}{\textwidth}{|>{\itshape}X|}
\hline
\textbf{Instruction} \\\hline
Given a piece of code that includes the repository name, file path, import statement, and code context, retrieve the function code from the same repository (but a different file). This function should be one that is used in the next line and has been imported in the provided import statement.
\\\hline
\textbf{Query} \\\hline
\texttt{\#\# repo\_name=vmagamedov/kinko} \newline
  \texttt{\#\# file\_path=kinko/checker.py} \newline
  \texttt{\#\# import\_statement} \newline
  \texttt{from itertools import chain} \newline
  \hspace*{2em} \texttt{from contextlib import contextmanager} \newline
  \hspace*{2em} \texttt{from collections import namedtuple, deque, defaultdict} \newline
  \hspace*{2em} \texttt{from .refs import ArgRef, FieldRef, ItemRef, Reference, is\_from\_arg, CtxRef} \newline
  \hspace*{2em} \texttt{from .nodes import Tuple, Number, Keyword, String, List, Symbol, Placeholder} \newline
  \colorbox{mediumgray}{\textup{[...]}} \newline
  \newline
  \texttt{\#\# code\_context} \newline
  \texttt{NamedArg['then',} \newline
  \hspace*{2em} \texttt{\_\_var.then\_],} \newline
  \texttt{NamedArg['else',} \newline
  \hspace*{2em} \texttt{\_\_var.else\_]],} \newline
  \colorbox{mediumgray}{\textup{[...]}} \newline
  \hspace*{2em} \texttt{\_\_var.result]} \newline
\\\hline

\textbf{Relevant Document} \\\hline
\texttt{class VarArgs(with\_metaclass(VarArgsMeta, object)):}\newline
\hspace*{2em} \texttt{pass}
\\\hline
\end{xltabular}
\end{center}

\subsubsection{SWE-Bench}

\begin{center}\small
\begin{xltabular}{\textwidth}{|>{\itshape}X|}
\hline
\textbf{Instruction} \\\hline
Given the description of an issue in the GitHub repository astropy, retrieve all files from the same repository that need to be updated in order to resolve the issue.
\\\hline
\textbf{Query} \\\hline
astropy.time.TimeDelta should support conversion to `datetime.timedelta`\newline
Because of the inheritance `TimeDelta` has a method `to\_datetime` which is useless.\newline\newline
It should have a method `to\_timedelta` which returns a `datetime.timedelta` object or objects.\newline
Conversion to `np.datetime64` (for `Time`) and `np.timedelta64` (for `TimeDelta`) would also be great.
\\\hline
\textbf{Relevant Document} \\\hline
\texttt{astropy/time/formats.py} \newline
  \texttt{\# -*- coding: utf-8 -*-} \newline
  \texttt{\# Licensed under a 3-clause BSD style license - see LICENSE.rst} \newline
  \newline
  \texttt{import fnmatch} \newline
  \texttt{import time} \newline
  \texttt{import re} \newline
  \texttt{import datetime} \newline
  \texttt{from collections import OrderedDict, defaultdict} \newline
  \newline
  \texttt{import numpy as np} \newline
  \newline
  \texttt{from ..utils.decorators import lazyproperty} \newline
  \texttt{from .. import units as u} \newline
  \texttt{from .. import \_erfa as erfa} \newline
  \texttt{from .utils import day\_frac, two\_sum} \newline
  \newline
  \texttt{\_\_all\_\_ = ['TimeFormat', 'TimeJD', 'TimeMJD', 'TimeFromEpoch', 'TimeUnix',} \newline
  \hspace*{1.5em} \texttt{'TimeCxcSec', 'TimeGPS', 'TimeDecimalYear',} \newline
  \hspace*{1.5em} \texttt{'TimePlotDate', 'TimeUnique', 'TimeDatetime', 'TimeString',} \newline
  \hspace*{1.5em} \texttt{'TimeISO', 'TimeISOT', 'TimeFITS', 'TimeYearDayTime',} \newline
  \hspace*{1.5em} \texttt{'TimeEpochDate', 'TimeBesselianEpoch', 'TimeJulianEpoch',} \newline
  \hspace*{1.5em} \texttt{'TimeDeltaFormat', 'TimeDeltaSec', 'TimeDeltaJD',} \newline
  \hspace*{1.5em} \texttt{'TimeEpochDateString', 'TimeBesselianEpochString',} \newline
  \hspace*{1.5em} \texttt{'TimeJulianEpochString', 'TIME\_FORMATS', 'TIME\_DELTA\_FORMATS',} \newline
  \hspace*{1.5em} \texttt{'TimezoneInfo']}\newline
  \colorbox{mediumgray}{\textup{[...]}}
\\\hline
\end{xltabular}
\end{center}

\subsection{Finance}

\subsubsection{Apple}

\begin{center}\small
\begin{xltabular}{\textwidth}{|>{\itshape}X|}
\hline
\textbf{Instruction} \\\hline
Given a finance-related question, retrieve relevant passages from Apple's 2022 SEC filings that provide the answer.
\\\hline
\textbf{Query} \\\hline
What is the aggregate market value of the voting and non-voting stock held by non-affiliates of the Registrant, as of March 25, 2022?
\\\hline
\textbf{Relevant Document} \\\hline
under Section 404(b) of the Sarbanes-Oxley Act (15 U.S.C. 7262(b)) by the registered public accounting firm that prepared or issued its audit report. \newline
Indicate by check mark whether the Registrant is a shell company (as defined in Rule 12b-2 of the Act). \newline
Yes  $\square$     No  $\boxtimes$ \newline
The aggregate market value of the voting and non-voting stock held by non-affiliates of the Registrant, as of March 25, 2022, the last business day of the Registrant’s most recently
\\\hline
\end{xltabular}
\end{center}

\subsubsection{ConvFinQA}

\begin{center}\small
\begin{xltabular}{\textwidth}{|>{\itshape}X|}
\hline
\textbf{Instruction} \\\hline
In a conversational finance question-answering task, given a list of questions, retrieve passages that contain the answer to the last question. Relevant passages should be sourced from finance reports, as specified by the file name in the query. These passages can be either a text excerpt or a table row.
\\\hline
\textbf{Query} \\\hline
File: LMT/2017/page\_80.pdf\newline
Dialogue:\newline
what was the total weighted average common shares outstanding for diluted computations in 2016 and 2017?\newline
and including the value for 2015?\newline
so what was the average during this time?\newline
how much did the weighted average common shares outstanding for diluted computations change between 2016 and 2017?
\\\hline
\textbf{Relevant Document} \\\hline
File: LMT/2017/page\_80.pdf\newline
Table row-3\newline
Header: ['', '2017', '2016', '2015']\newline
['weighted average common shares outstanding for diluted computations', '290.6', '303.1', '314.7']
\\\hline
\end{xltabular}
\end{center}

\subsubsection{FinanceBench}
\begin{center}\small
\begin{xltabular}{\textwidth}{|>{\itshape}X|}
\hline
\textbf{Instruction} \\\hline
Given a question about publicly traded companies, retrieve pages from the specified file that contain the answer to the question.
\\\hline
\textbf{Query} \\\hline
File: 3M\_2018\_10K.pdf\newline
Question: What is the FY2018 capital expenditure amount (in USD millions) for 3M? Give a response to the question by relying on the details shown in the cash flow statement.
\\\hline
\textbf{Relevant Document} \\\hline
File: 3M\_2018\_10K.pdf\newline
Page: 85\newline
Table of Contents\newline
3M Company and Subsidiaries Consolidated Statement of Cash Flows Years ended December 31 (Millions)\newline
{\tiny
\begin{tabular}{|p{10cm}|p{1cm}|p{1cm}|p{1cm}|}
\hline
 & \texttt{2018} & \texttt{2017} & \texttt{2016} \\
\hline
\texttt{Cash Flows from Operating Activities} & & & \\
\hline
\texttt{Net income including noncontrolling interest} & \$ 5,363 & \$ 4,869 & \$ 5,058 \\
\hline
\texttt{Adjustments to reconcile net income including noncontrolling interest to net cash provided by operating activities} & & & \\
\hline
\texttt{Depreciation and amortization} & 1,488 & 1,544 & 1,474 \\
\hline
\texttt{Company pension and postretirement contributions} & (370) & (967) & (383) \\
\hline
\texttt{Company pension and postretirement expense} & 410 & 334 & 250 \\
\hline
\texttt{Stock-based compensation expense} & 302 & 324 & 298 \\
\hline
\texttt{Gain on sale of businesses} & (545) & (586) & (111) \\
\hline
\texttt{Deferred income taxes} & (57) & 107 & 7 \\
\hline
\texttt{Changes in assets and liabilities} & & & \\
\hline
\texttt{Accounts receivable} & (305) & (245) & (313) \\
\hline
\texttt{Inventories} & (509) & (387) & 57 \\
\hline
\texttt{Accounts payable} & 408 & 24 & 148 \\
\hline
\texttt{Accrued income taxes (current and long-term)} & 134 & 967 & 101 \\
\hline
\texttt{Other — net} & 120 & 256 & 76 \\
\hline
\texttt{Net cash provided by (used in) operating activities} & 6,439 & 6,240 & 6,662 \\
\hline
\colorbox{mediumgray}{\textup{[...]}}&&&\\
\hline
\texttt{Net increase (decrease) in cash and cash equivalents} & (200) & 655 & 600 \\
\hline
\texttt{Cash and cash equivalents at beginning of year} & 3,053 & 2,398 & 1,798 \\
\hline
\texttt{Cash and cash equivalents at end of period} & \$ 2,853 & \$ 3,053 & \$ 2,398 \\
\hline
\end{tabular}
}

The accompanying Notes to Consolidated Financial Statements are an integral part of this statement. 60
\\\hline
\end{xltabular}
\end{center}

\subsubsection{FinQA}

\begin{center}\small
\begin{xltabular}{\textwidth}{|>{\itshape}X|}
\hline
\textbf{Instruction} \\\hline
Given a question and a specified file name, retrieve relevant passages that contain the answer to the question. The relevant passages can be either text excerpts or table rows from the specified file.
\\\hline
\textbf{Query} \\\hline
File: ETR/2016/page\_23.pdf\newline
Question:\newline
what is the growth rate in net revenue in 2015 for entergy corporation?
\\\hline
\textbf{Relevant Document} \\\hline
File: ETR/2016/page\_23.pdf\newline
Table row-1\newline
Header: ['', 'amount ( in millions )']\newline
['2014 net revenue', '\$ 5735']
\\\hline
\end{xltabular}
\end{center}

\subsubsection{HC3Finance}

\begin{center}\small
\begin{xltabular}{\textwidth}{|>{\itshape}X|}
\hline
\textbf{Instruction} \\\hline
Given a finance-related question, retrieve the most accurate and relevant answer.
\\\hline
\textbf{Query} \\\hline
Should the poor consider investing as a means to becoming rich?
\\\hline
\textbf{Relevant Document} \\\hline
What could a small guy with \$100 do to make himself not poor To answer the question directly, not much. Short of investing in something at the exact moment before it goes bananas, then reinvesting into a bigger stock and bigger etc, it's super high risk. A better way is to sacrifice some small things, less coffee, less smokes, less going out partying so that instead of having \$100, you have \$100 a week. This puts you into a situation where you can save enough to become a deposit on an appreciating asset (choose your own asset class, property in AU for me). Take out a loan for as much as you can for your \$100 a week payment and make it interest only with an offset against it, distributions from shares can either be reinvested or put into the offset or in the case of property, rent can be put against the offset, pretty soon you end up with a scenario where you have cash offsetting a loan down to nothing but you still have access to the cash, invest into another place and revalue your asset, you can take out any equity that has grown and put that also into your offset. Keep pulling equity and using the money from the offset as deposits on other assets (it kind of works really well on property) and within 15 years you can build an empire with a passive income to retire on. The biggest thing the rich guys get that the poor guys don't is that debt is GOOD, use someone else's money to buy an appreciating asset then when you pay it back eventually, you own the growth. Use debt to buy more debt for exponential growth. Of course, you need to also invest your time to research what you are investing in, you need to know when you make the decision to buy that it will appreciate, it's no good just buying off a tip, you may as well drop your money on the horses if you want to play it like that. Fortunately, one thing we all have in common regardless of our money is time, we have time which we can invest.
\\\hline
\end{xltabular}
\end{center}

\subsubsection{TAT-DQA}

\begin{center}\small
\begin{xltabular}{\textwidth}{|>{\itshape}X|}
\hline
\textbf{Instruction} \\\hline
Given a question, retrieve a paragraph from the specified financial report that contains or can infer the answer.
\\\hline
\textbf{Query} \\\hline
File: bce-inc\_2019.pdf\newline
What is the \% change in the capital intensity ratio for BCE?
\\\hline
\textbf{Relevant Document} \\\hline
File: bce-inc\_2019.pdf\newline
Page: 0\newline
Chunk 5\newline
Bell Wireline 3,183 3,193 10 0.3\% Capital intensity ratio 25.8\% 26.0\% 0.2 pts\newline
Bell Media 108 114 6 5.3\% Capital intensity ratio 3.4\% 3.7\% 0.3 pts\newline
BCE 3,988 3,971 (17) (0.4\%) Capital intensity ratio 16.6\% 16.9\% 0.3 pts\newline
BCE capital expenditures totaled \$3,988 million for the year, up \$17 million over 2018. This corresponded to a capital intensity ratio of 16.6\%, down 0.3 pts compared to last year. Capital spending in the year reflected the following:\newline
- Greater capital investments in our wireless segment of \$33 million
\\\hline
\end{xltabular}
\end{center}

\subsubsection{Trade-the-event}

\begin{center}\small
\begin{xltabular}{\textwidth}{|>{\itshape}X|}
\hline
\textbf{Instruction} \\\hline
Retrieve the full document for a finance news article based on its title.
\\\hline
\textbf{Query} \\\hline
Investor Alert: Kaplan Fox Investigates Potential Securities Fraud At QuantumScape Corporation
\\\hline
\textbf{Relevant Document} \\\hline
NEW YORK, Jan. 7, 2021 /PRNewswire/ -- Kaplan Fox \& Kilsheimer LLP (www.kaplanfox.com) is investigating claims on behalf of investors of QuantumScape Corporation (``QuantumScape'' or the ``Company'') (NYSE: QS).\newline
A complaint has been filed on behalf of investors who purchased QuantumScape securities between November 27, 2020 and December 31, 2020, inclusive (the ``Class Period'').\newline
According to the complaint, throughout the Class Period the defendants made materially false and misleading statements and omitted to disclose that QuantumScape's battery technology was not sufficient for electric vehicle performance as it would not be able to withstand the aggressive automotive environment and likely provided no meaningful improvement over existing battery technology.\newline
On January 4, 2021, Seeking Alpha published an article alleging that several risks associated with QuantumScape's solid-state batteries made them ``completely unacceptable for real world field electric vehicles.''\newline
Following the publication of the Seeking Alpha article, QuantumScape's stock price fell \$34.39 per share, over 40\%, to close at \$49.96 per share on January 3, 2021.\newline
\colorbox{mediumgray}{\textup{[...]}}
\\\hline
\end{xltabular}
\end{center}

\subsubsection{FiQA}

\begin{center}\small
\begin{xltabular}{\textwidth}{|>{\itshape}X|}
\hline
\textbf{Instruction} \\\hline
Given a financial question, retrieve user replies that best answer the question.
\\\hline
\textbf{Query} \\\hline
How to account for money earned and spent prior to establishing business bank accounts?
\\\hline
\textbf{Relevant Document} \\\hline
Funds earned and spent before opening a dedicated business account should be classified according to their origination. For example, if your business received income, where did that money go?  If you took the money personally, it would be considered either a 'distribution' or a 'loan' to you.  It is up to you which of the two options you choose. On the flip side, if your business had an expense that you paid personally, that would be considered either a 'contribution of capital' or a 'loan' from you. If you choose to record these transactions as loans, you can offset them together, so you don't need two separate accounts, loan to you and loan from you. When the bank account was opened, the initial deposit came from where?  If it came from your personal funds, then it is either a 'contribution of capital' or a 'loan' from you. From the sound of your question, you deposited what remained after the preceding income/expenses.  This would, in effect, return the 'loan' account back to zero, if choosing that route. The above would also be how to record any expenses you may pay personally for the business (if any) in the future. Because these transactions were not through a dedicated business bank account, you can't record them in Quickbooks as checks and deposits.  Instead, you can use Journal Entries.  For any income received, you would debit your capital/loan account and credit your income account.  For any expenses, you would debit the appropriate expense account and credit your distribution/loan account. Also, if setting up a loan account, you should choose either Current Asset or Current Liability type.  The capital contribution and distribution account should be Equity type. Hope this helps!
\\\hline
\end{xltabular}
\end{center}

\subsection{Web}

\subsubsection{ELI5}

\begin{center}\small
\begin{xltabular}{\textwidth}{|>{\itshape}X|}
\hline
\textbf{Instruction} \\\hline
Given a question, retrieve passages from Wikipedia that can help answer the question.
\\\hline
\textbf{Query} \\\hline
In Trading Places (1983, Akroyd/Murphy) how does the scheme at the end of the movie work? Why would buying a lot of OJ at a high price ruin the Duke Brothers?
\\\hline
\textbf{Relevant Document} \\\hline
Content: Trading Places is a 1983 American comedy film directed by John Landis and starring Dan Aykroyd and Eddie Murphy. It tells the story of an upper-class commodities broker and a homeless street hustler whose lives cross paths when they are unknowingly made part of an elaborate bet. Ralph Bellamy, Don Ameche, Denholm Elliott, and Jamie Lee Curtis also star. The storyline is often called a modern take on Mark Twain's classic 19th-century novel \"The Prince and the Pauper\".
\\\hline
\end{xltabular}
\end{center}

\subsubsection{Fever}

\begin{center}\small
\begin{xltabular}{\textwidth}{|>{\itshape}X|}
\hline
\textbf{Instruction} \\\hline
Given a claim, retrieve passages from Wikipedia that support or refute the claim.
\\\hline
\textbf{Query} \\\hline
One True Thing is an American film.
\\\hline
\textbf{Relevant Document} \\\hline
Content: One True Thing is a 1998 American drama film directed by Carl Franklin. It tells the story of a woman who is forced to put her life on hold in order to care for her mother who is dying of cancer. It was adapted by Karen Croner from the novel by Anna Quindlen. The novel and film are based on Anna Quindlen's real life struggle with the death of her mother, Prudence Pantano Quindlen, from ovarian cancer in 1972.
\\\hline
\end{xltabular}
\end{center}

\subsubsection{AY2}

\begin{center}\small
\begin{xltabular}{\textwidth}{|>{\itshape}X|}
\hline
\textbf{Instruction} \\\hline
In this entity linking task, you are given a paragraph containing a single entity mention, which is marked by two special tokens: [START\_ENT] and [END\_ENT]. Your task is to retrieve the relevant Wikipedia page for the tagged entity mention.
\\\hline
\textbf{Query} \\\hline
CRICKET - LEICESTERSHIRE TAKE OVER AT TOP AFTER INNINGS VICTORY .  LONDON 1996-08-30  West Indian all-rounder Phil Simmons took four for 38 on Friday as Leicestershire beat Somerset by an innings and 39 runs in two days to take over at the head of the county championship .  Their stay on top , though , may be short-lived as title rivals Essex , Derbyshire and Surrey all closed in on victory while Kent made up for lost time in their rain-affected match against Nottinghamshire .  After bowling Somerset out for 83 on the opening morning at Grace Road , Leicestershire extended their first innings by 94 runs before being bowled out for 296 with England discard Andy Caddick taking three for 83 .  Trailing by 213 , [START\_ENT] Somerset [END\_ENT] got a solid start to their second innings before Simmons stepped in to bundle them out for 174 .  Essex , however , look certain to regain their top spot after Nasser Hussain and Peter Such gave them a firm grip on their match against Yorkshire at Headingley .  Hussain , considered surplus to England 's one-day requirements , struck 158 , his first championship century of the season , as Essex reached 372 and took a first innings lead of 82 .  \colorbox{mediumgray}{\textup{[...]}}
\\\hline
\textbf{Relevant Document} \\\hline
Content: Somerset County Cricket Club is one of eighteen first-class county clubs within the domestic cricket structure of England and Wales. It represents the historic county of Somerset. Founded in 1875, Somerset was initially regarded as a minor county until official first-class status was gained in 1895. Somerset has competed in the County Championship since 1891 and has subsequently played in every top-level domestic cricket competition in England. The club's limited overs team was formerly named the Somerset Sabres, but is now known only as Somerset.
\\\hline
\end{xltabular}
\end{center}

\subsubsection{WnCw}

\begin{center}\small
\begin{xltabular}{\textwidth}{|>{\itshape}X|}
\hline
\textbf{Instruction} \\\hline
In this entity linking task, you are given a paragraph containing a single entity mention, which is marked by two special tokens: [START\_ENT] and [END\_ENT]. Your task is to retrieve the relevant Wikipedia page for the tagged entity mention.
\\\hline
\textbf{Query} \\\hline
\colorbox{mediumgray}{\textup{[...]}}
In text import import wizard  Choose Delimited if the data are delimited and  Fixed width if the  data are fixed width .  In this example either option can be chosen .  Set the Start import at row to the first row that  has data , skipping any preceding text such as explanation of the data .  In this example there is now preceding text , so Start  import at row 1 .  So Step 1 : choose [START\_ENT] Delimited [END\_ENT] and Start Import at Row  1 and hit Next .  This yields Step 2 .  The default Delimiter is Tab .  Change this to Space .  Then check that the Data preview has correctly split up the data , as is  the case below .  Hit next .  This yields step 3 .  In this case leave the column data format as  general .  Hit Finish .  This should give you an Excel worksheet with 2 columns and 5 rows in  cells A1 
\\\hline
\textbf{Relevant Document} \\\hline
Content: Formats that use delimiter-separated values (also DSV) store two-dimensional arrays of data by separating the values in each row with specific delimiter characters. Most database and spreadsheet programs are able to read or save data in a delimited format. Due to their wide support, DSV files can be used in data exchange among many applications.
\\\hline
\end{xltabular}
\end{center}

\subsubsection{WnWi}

\begin{center}\small
\begin{xltabular}{\textwidth}{|>{\itshape}X|}
\hline
\textbf{Instruction} \\\hline
In this entity linking task, you are given a paragraph containing a single entity mention, which is marked by two special tokens: [START\_ENT] and [END\_ENT]. Your task is to retrieve the relevant Wikipedia page for the tagged entity mention.
\\\hline
\textbf{Query} \\\hline
Robin \" Bob \" Coverdale (birth registered October $\rightarrow$ December in Sculcoates district) is an English professional Rugby League World Cup winning footballer of the 1950s and '60s, playing at representative level for Great Britain, and at club level for Hull, Wakefield Trinity, and Hull Kingston Rovers, as a, i.e. number 8 or 10, during the era of. Bob Coverdale won caps for Great Britain while at Hull in the 1954 Rugby League World Cup against Australia, France, New Zealand, and France. Bob Coverdale played Right -, i.e. number 10 in all four of Great Britain's 1954 Rugby League World Cup matches, including Great Britain's 16-12 victory over France in the 1954 Rugby League World Cup final at Parc des Princes, Paris on Saturday 13 November 1954. Bob Coverdale played in all three of Hull's defeats in the 1953--54, 1954--55, and [START\_ENT] 1955--56 [END\_ENT] Yorkshire Cup.
\\\hline
\textbf{Relevant Document} \\\hline
Content: The 1955--56 Rugby Football League season was the 61st season of rugby league football.
\\\hline
\end{xltabular}
\end{center}

\subsubsection{TREx}

\begin{center}\small
\begin{xltabular}{\textwidth}{|>{\itshape}X|}
\hline
\textbf{Instruction} \\\hline
Given a structured input in the form of 'subject entity [SEP] relation,' retrieve Wikipedia passages that contain the object entities and confirm the subject-relation-object fact.
\\\hline
\textbf{Query} \\\hline
Death SS [SEP] genre
\\\hline
\textbf{Relevant Document} \\\hline
Content: Death SS (later also intended as a contraction of In Death of Steve Sylvester) is an Italian heavy metal band.
\\\hline
\end{xltabular}
\end{center}

\subsubsection{zsRE}

\begin{center}\small
\begin{xltabular}{\textwidth}{|>{\itshape}X|}
\hline
\textbf{Instruction} \\\hline
Given a structured input in the form of 'subject entity [SEP] relation,' retrieve Wikipedia passages that contain the object entities and confirm the subject-relation-object fact.
\\\hline
\textbf{Query} \\\hline
USA-5 [SEP] time of spacecraft launch
\\\hline
\textbf{Relevant Document} \\\hline
Content: USA-5, also known as Navstar 10, GPS I-10 and GPS SVN-10, was an American navigation satellite launched in 1984 as part of the Global Positioning System development programme. It was the tenth of eleven Block I GPS satellites to be launched.
\\\hline
\end{xltabular}
\end{center}

\subsubsection{WoW}

\begin{center}\small
\begin{xltabular}{\textwidth}{|>{\itshape}X|}
\hline
\textbf{Instruction} \\\hline
Given a conversation based on information retrieved from Wikipedia, retrieve relevant passages that can support the next utterance.
\\\hline
\textbf{Query} \\\hline
I love the 1980s music one of my favorite artists is michael jackson\newline
You mean all of the major events and trends in pop music in the 80s? I love 80s music!\newline
yes thriller was one of the best albums ever made every song was a hit\newline
Yeah Thriller was quite good, the 80s also saw the emergence of New Wave as a genre.\newline
what is the new wave genre. i have never heard of that\newline
New Wave was similar to Punk Rock but also included electronic elements, Tears for Fears is an example.\newline
i have never heard of tears for fears before. what where there singles.
\\\hline
\textbf{Relevant Document} \\\hline
Content: Tears for Fears are an English pop rock band formed in Bath, England in 1981 by Roland Orzabal and Curt Smith. Founded after the dissolution of their first band, the mod-influenced Graduate, Tears for Fears were initially associated with the new wave synthesiser bands of the early 1980s. Later, the band branched out into mainstream rock and pop and attained international chart success. Tears for Fears were part of the MTV-driven Second British Invasion of the US.
\\\hline
\end{xltabular}
\end{center}

\subsubsection{ArguAna}

\begin{center}\small
\begin{xltabular}{\textwidth}{|>{\itshape}X|}
\hline
\textbf{Instruction} \\\hline
Given a claim, find documents that refute the claim.
\\\hline
\textbf{Query} \\\hline
IBeing vegetarian helps the environment \newline
Becoming a vegetarian is an environmentally friendly thing to do. Modern farming is one of the main sources of pollution in our rivers. Beef farming is one of the main causes of deforestation, and as long as people continue to buy fast food in their billions, there will be a financial incentive to continue cutting down trees to make room for cattle. Because of our desire to eat fish, our rivers and seas are being emptied of fish and many species are facing extinction. Energy resources are used up much more greedily by meat farming than my farming cereals, pulses etc. Eating meat and fish not only causes cruelty to animals, it causes serious harm to the environment and to biodiversity. For example consider Meat production related pollution and deforestation \newline
At Toronto\u2019s 1992 Royal Agricultural Winter Fair, Agriculture Canada displayed two contrasting statistics: \u201cit takes four football fields of land (about 1.6 hectares) to feed each Canadian\u201d and \u201cone apple tree produces enough fruit to make 320 pies.\u201d Think about it \u2014 a couple of apple trees and a few rows of wheat on a mere fraction of a hectare could produce enough food for one person! [1] \colorbox{mediumgray}{\textup{[...]}}
\\\hline
\textbf{Relevant Document} \\\hline
animals environment general health health general weight philosophy ethics\\
You don’t have to be vegetarian to be green. Many special environments have been created by livestock farming – for example chalk down land in England and mountain pastures in many countries. Ending livestock farming would see these areas go back to woodland with a loss of many unique plants and animals. Growing crops can also be very bad for the planet, with fertilisers and pesticides polluting rivers, lakes and seas. Most tropical forests are now cut down for timber, or to allow oil palm trees to be grown in plantations, not to create space for meat production. British farmer and former editor Simon Farrell also states: “Many vegans and vegetarians rely on one source from the U.N. calculation that livestock generates 18\% of global carbon emissions, but this figure contains basic mistakes. It attributes all deforestation from ranching to cattle, rather than logging or development. It also muddles up one-off emissions from deforestation with on-going pollution.” He also refutes the statement of meat production inefficiency: “Scientists have calculated that globally the ratio between the amounts of useful plant food used to produce meat is about 5 to 1. If you feed animals only food that humans can eat – which is, indeed, largely the case in the Western world – that may be true. But animals also eat food we can't eat, such as grass. So the real conversion figure is 1.4 to 1.” At the same time eating a vegetarian diet may be no more environmentally friendly than a meat-based diet if it is not sustainably sourced or uses perishable fruit and vegetables that are flown in from around the world. Eating locally sourced food can have as big an impact as being vegetarian. 
\\\hline
\end{xltabular}
\end{center}

\subsubsection{CQADupStack}

\begin{center}\small
\begin{xltabular}{\textwidth}{|>{\itshape}X|}
\hline
\textbf{Instruction} \\\hline
Retrieve duplicate questions from StackOverflow forum.
\\\hline
\textbf{Query} \\\hline
Turn a Android Phone with broken screen into dedicated Web server
\\\hline
\textbf{Relevant Document} \\\hline
Setting up web server on flooded HTC Wildfire S\newline
A couple of months ago I got my Wildfire S accidentally flooded. It was just collecting dust since then, but today I came up with an idea to get a web server running on it. As far as I know, everything works fine except the display. So here's my question: is there a way to set up a server on that phone without the need to use the touchscreen? Maybe I could install some light linux distribution and configure it via USB/SSH? Thanks!

\\\hline
\end{xltabular}
\end{center}

\subsubsection{Quora}

\begin{center}\small
\begin{xltabular}{\textwidth}{|>{\itshape}X|}
\hline
\textbf{Instruction} \\\hline
Given a question, retrieve questions that are semantically equivalent to the given question.
\\\hline
\textbf{Query} \\\hline
Which question should I ask on Quora?
\\\hline
\textbf{Relevant Document} \\\hline
What are good questions to ask on Quora?
\\\hline
\end{xltabular}
\end{center}

\subsubsection{TopiOCQA}

\begin{center}\small
\begin{xltabular}{\textwidth}{|>{\itshape}X|}
\hline
\textbf{Instruction} \\\hline
In conversational information seeking, given a dialogue, retrieve passages from Wikipedia to asnwer the last question.
\\\hline
\textbf{Query} \\\hline
Dialogue Context:\newline
when will the new dunkirk film be released on dvd\newline
18 December 2017\newline
what is this film about?\newline
Dunkirk evacuation of World War II\newline
\colorbox{mediumgray}{\textup{[...]}}
are whales captured here?\newline
Whaling was an important economic activity from the 9th until the 13th century by by 1902 the whaling had ended\newline
any particular whale species that was hunted?\newline
Gray whale\newline
Question: where are they found?
\\\hline
\textbf{Relevant Document} \\\hline
Gray whale [SEP] Introduction\newline
This mammal is descended from filter-feeding whales that appeared at the beginning of the Oligocene, over 30 million years ago. The gray whale is distributed in an eastern North Pacific (North American), and an endangered western North Pacific (Asian), population. North Atlantic populations were extirpated (perhaps by whaling) on the European coast before AD 500, and on the American coast around the late 17th to early 18th centuries. Even so, on May 8, 2010, a sighting of a gray whale was confirmed off the coast of Israel in the Mediterranean Sea, leading some scientists to think they might be repopulating old breeding grounds that have not been visited for centuries.
\\\hline
\end{xltabular}
\end{center}

\subsubsection{Touche}
\begin{center}\small
\begin{xltabular}{\textwidth}{|>{\itshape}X|}
\hline
\textbf{Instruction} \\\hline
Given a query, retrieve documents that answer the query.
\\\hline
\textbf{Query} \\\hline
Should teachers get tenure?
\\\hline
\textbf{Relevant Document} \\\hline
Colleges should abolish the ability for teachers to be tenured.\newline
Since I assume their opening statement was made in their R1 post, I will begin mine as well. I will be arguing against the idea that tenure for college professors should be abolished. I have three main claims: [Claim 1]: Tenure is a necessity [Claim 2]: Tenured teachers can still be fired (and other misconceptions) [Claim 3]: Research supports tenure [C1]: Tenure is a necessity The concept of tenure dates back over 100 years ago to the early 20 century, when working in the field of education was much different than what it is today [1]. It was female-dominated, classrooms were larger, and working conditions were poorer [2]. Before tenure, teachers could be fired for any reason. If a teacher had the audacity to get married or, even more horrific, pregnant, the schoolboard could immediately fire her. Tenure and teachers' unions were created to guarantee some amount of job protection for teachers. They wanted the peace of mind to know their job wouldn't be terminated for seemingly no reason. At the high school level, most schools require teachers work at the same school for 3-5 years before being considered for tenure, and there are many factors taken into account, with the most important . \colorbox{mediumgray}{\textup{[...]}}
\\\hline
\end{xltabular}
\end{center}

\subsubsection{ACORDAR}

\begin{center}\small
\begin{xltabular}{\textwidth}{|>{\itshape}X|}
\hline
\textbf{Instruction} \\\hline
Given a question, identify and retrieve datasets where the keywords in the query may be found in either the metadata or the actual data of the dataset.
\\\hline
\textbf{Query} \\\hline
What datasets are available on patent infringement lawsuits filed in a specific industry or region?
\\\hline
\textbf{Relevant Document} \\\hline
\{'license': 'License not specified', \\
'size': 'None', \\
'created': '2015-01-30T17:03:21.241594', \\
'dataset\_id': '1174', \\
'description': 'Bills Signed By Governor Kitzhaber 2014', \\
'title': 'Bills Signed By Governor Kitzhaber 2014', \\
'tags': ''\}
\\\hline
\end{xltabular}
\end{center}

\subsubsection{CPCD}

\begin{center}\small
\begin{xltabular}{\textwidth}{|>{\itshape}X|}
\hline
\textbf{Instruction} \\\hline
The query is a dialogue history in which the user seeks music recommendations. In each turn, the system recommends some music, and the user provides feedback indicating whether they like or dislike the recommendations. Based on the user's preferences and requests, retrieve music that the user is likely to enjoy as the recommendation response.
\\\hline
\textbf{Query} \\\hline
User: I need a breakup playlist full of depressing songs please\newline
System: any specific genres or artists?\newline
User Feedback: I like these: Only Love Can Break Your Heart. And I dislike these: Hurt, SAD!\newline
User: Love the Neil Young but not a Johnny Cash fan - how about some pop songs?\newline
System: Here are some songs to try!\newline
User Feedback: I like these: Don't Speak, Someone Like You, Torn. And I dislike these: Back To Black, Ordinary People\newline
User: Great! How about some of the darker British New Wave stuff - The Cure or Echo and the Bunnymen?\newline
System: I am learning some new music thanks to you! I have added some songs how are these?\newline
User Feedback: I like these: Cold (Remastered Version), The Killing Moon, Gone, Gone, Gone. And I dislike these: Catch (2006 Remaster), Lips Like Sugar, Lovesong\newline
User: Awesome! Ok let's get to the angry part - how about some Elvis Costello and Chris Isaak?\newline
System: Sure thing! Whats the next step in the healing process?!\newline
User Feedback: I like these: Baby Did a Bad Bad Thing, Somebody's Crying, I'm Not Angry, Wicked Game, Lie To Me. And I dislike these: Radio, Radio (2021 Remaster), When I Was Cruel No.2, Less Than Zero\newline
User: Let's skip on to the post breakup new relationship phase! How about some happy, bouncy stuff? :)
\\\hline
\textbf{Relevant Document} \\\hline
\{'track\_titles': \"Let's Go Crazy\", 'track\_release\_titles': 'Purple Rain', 'track\_artists': ['Prince and the Revolution'], 'track\_canonical\_ids': 'C04P6W8MDBg'\}
\\\hline
\end{xltabular}
\end{center}

\subsubsection{ChroniclingAmericaQA}

\begin{center}\small
\begin{xltabular}{\textwidth}{|>{\itshape}X|}
\hline
\textbf{Instruction} \\\hline

\\\hline
\textbf{Query} \\\hline

\\\hline
\textbf{Relevant Document} \\\hline

\\\hline
\end{xltabular}
\end{center}

\begin{center}\small
\begin{xltabular}{\textwidth}{|>{\itshape}X|}
\hline
\textbf{Instruction} \\\hline
Given a question, retrieve newspaper pages that contain the answer of the question from American historical newspaper dataset Chronicling America
\\\hline
\textbf{Query} \\\hline
How many acres is the Salem Laundry Co. on South Liberty Street?
\\\hline
\textbf{Relevant Document} \\\hline
Has only a few acres in cultivation, with about 10 acres cleared. The wood and piling timber on this is worth all they ask for the place. It is a special bargain at \$50 per acre. Yours, COURTIER \& VICE, 143 S. Liberty Street. Promptness is another point. On one of our good, if we promise your package for a certain time, you'll have it at that time. We use a system that enables us to tell just when an article will be completely laundered, and we make no promises that we cannot fulfill. Do you get perfect work and get it always on time? If not, try us. Salem Laundry Co., 1 Md-160 South Liberty Street, Telephone Main 58.
\\\hline
\end{xltabular}
\end{center}

\subsubsection{NTCIR}

\begin{center}\small
\begin{xltabular}{\textwidth}{|>{\itshape}X|}
\hline
\textbf{Instruction} \\\hline
Given a search query, retrieve relevant datasets from Data.gov and e-Stat that contain the requested information.
\\\hline
\textbf{Query} \\\hline
oysters dislike east coast
\\\hline
\textbf{Relevant Document} \\\hline
The Millennium Challenge Corporation (MCC) provided funds for the upgrade of two roads in Vanuatu.  These were the Efate Ring Road and the Santo East Coast Road.  Both these roads were unpaved (coral) roads and were sealed with a double surface dressing in 2009/10.  The length of road sealed in Efate was 92.5 km and 57.2 km in Santo.  An HDM-4 analysis was conducted to examine:) The economic viability of upgrading the two roads   ii) The future performance of the roads
\\\hline
\end{xltabular}
\end{center}

\subsubsection{PointRec}

\begin{center}\small
\begin{xltabular}{\textwidth}{|>{\itshape}X|}
\hline
\textbf{Instruction} \\\hline
Given a user's request, recommend a point of interest (POI) that best matches the user's intent. Use the following metadata for reference: \{'Group': 'I', 'Main Category': 'Arts \& Entertainment', 'Sub Categories': ['Museums', 'Art Galleries', 'Castles'], 'Constraints\_text': ['I like museums, castles, art galleries, night life, monuments.'], 'Constraints': \{'NICE\_TO': ['museums', 'castles', 'art galleries', 'monuments']\}, 'Request\_text': ['Can anyone recommend attractions to see?'], 'Request': ['attractions'], 'City': 'Munich', 'Country': 'DE', 'State': None\}
\\\hline
\textbf{Query} \\\hline
Travelling to Germany ! 10 points!!?\newline
Hi there, i will be travelling to Germany for 2 weeks in July. Berlin, Hamburg, Frankurt and Munich. Can anyone recommend attractions to see? I like museums, castles, art galleries, night life, monuments. thank you!
\\\hline
\textbf{Relevant Document} \\\hline
\{'name': 'New Pinakothek', \newline
'alias': 'neue-pinakothek-münchen', \newline
'main\_category': 'Arts \& Entertainment', \newline
'sub\_categories': 'Art Museums, ', \newline
'rating': 4.0, 'price': None, 'address': 'Barer Str. 29', 'city\_from\_postal': 'Kreisfreie Stadt München', 'city': 'Munich', 'zip\_code': '80799', 'country\_code': 'DE', 'state\_code': 'BY', 'phone': '+498923805195', 'review\_count': 43, 
\newline
'snippets': [\{'url': 'https://www.pinakothek.de/en/visit/neue-pinakothek', \newline
'snippet': 'Neue Pinakothek “Rediscover the 19th Century” is the motto of the Neue Pinakothek. A richly varied tour provides an opportunity to view paintings and sculptures of the Neoclassical, Romantic, Impressionist, Art Nouveau and Gründerzeit periods and to encounter masterpieces by major pioneers of Modern art: Max Liebermann, Edouard Manet, Claude Monet, Vincent van Gogh and Paul Cézanne.', \newline
'title': 'Neue Pinakothek | DIE PINAKOTHEKEN', \newline
'family\_friendly': 1\}, \newline
\colorbox{mediumgray}{\textup{[...]}}\newline
\{'url': 'https://www.pinakothek.de/en/visit', \newline
'snippet': 'PREVENTION MEASURES: CLOSED FROM MARCH 14th ON In view of the dynamic spread of the coronavirus SARS-CoV-2, the Alte Pinakothek and Pinakothek der Moderne, the Museum Brandhorst, the Schack Collection and all state galleries will be closed to the public from March 14, initially until the end of the Easter holidays (April 20).', \newline
'title': 'Visit | DIE PINAKOTHEKEN', \newline
'family\_friendly': 1\}]\}
\\\hline
\end{xltabular}
\end{center}

\subsubsection{ProCIS-Dialog}

\begin{center}\small
\begin{xltabular}{\textwidth}{|>{\itshape}X|}
\hline
\textbf{Instruction} \\\hline
Given a multi-party human conversation (such as a Reddit post and its comments), retrieve relevant documents from Wikipedia to provide contextual information. The criteria for relevance are as follows:\newline
- Relevance: The document is directly related to the conversation, providing substantial useful context, background, or additional information that enhances the understanding of the conversation. This includes articles about the main topic, key individuals, events, or concepts mentioned in the conversation.\newline
- Partially Relevant: The document is somewhat related to the conversation. It may provide some context or additional information but is not directly tied to the main topic of the conversation. This includes articles about broader themes, tangential topics, or peripheral concepts mentioned in the conversation.\newline
- Irrelevant: The document is not related to the conversation in any way. It does not provide any useful context or additional information to the conversation.
\\\hline
\textbf{Query} \\\hline
\textbf{Post} \newline
lolbacon: Why isn't the reddit alien dressed like Thriller-era Michael Jackson? \newline
Seriously guys, the fuck? \newline
\textbf{Thread} \newline
watso4183: I'd rather see it in a prison jump suit. Anyone else forgetting the terrible things this man did? \newline
dhaggerfin: Enlighten us with sources please. \newline
watso4183: Your kidding me right? \newline
dhaggerfin: From wikipedia: \newline
> Jackson was accused of child sexual abuse by a 13-year-old child named Jordan Chandler and his father Evan Chandler. Sometime afterwards, Evan Chandler was tape-recorded saying amongst other things, "If I go through with this, I win big-time. There's no way I lose. I will get everything I want and they will be destroyed forever...Michael's career will be over". A year after they had met, under the influence of a controversial sedative, Jordan Chandler told his father that Jackson had touched his penis. \newline
You tell me what that sounds like. Oh, and how about the MILLIONS of dollars he donated to charity: \newline
> He donated his \$5 million share from the Victory Tour to charity colorbox{mediumgray}{\textup{[...]}}
\\\hline
\textbf{Relevant Document} \\\hline
Timeline\_of
\_Reddit\newline
This is a timeline of Reddit, an entertainment, social networking, and news website where registered community members can submit content, such as text posts or direct links, making it essentially an online bulletin board system. 
\\\hline
\end{xltabular}
\end{center}

\subsubsection{ProCIS-Turn}

\begin{center}\small
\begin{xltabular}{\textwidth}{|>{\itshape}X|}
\hline
\textbf{Instruction} \\\hline
Given a multi-party human conversation (such as a Reddit post and its comments), retrieve relevant documents for the following utterance in the thread to provide contextual information: Sabakunoneji: 42 is a green and blue.  I see multiple digit numbers as their individual colors side by side.  Same with pi\newline\newline
Criteria for Relevance:\newline
- Relevance: The document is directly related to the utterance, providing substantial useful context, background, or additional information that enhances the understanding of the utterance.\newline
- Partially Relevant: The document is somewhat related to the utterance. It may provide some context or additional information but is not directly tied to the main topic of the utterance.\newline
- Irrelevant: The document is not related to the utterance in any way. It does not provide any useful context or additional information to the utterance.
\\\hline
\textbf{Query} \\\hline
\textbf{Post}\newline
Sabakunoneji: I'm synesthetic. AMA\newline
\url{http://en.wikipedia.org/wiki/Synesthesia}\newline
I have grapheme -> color, sound -> color, and number form synesthesia. Ask away!\newline
\textbf{Thread}\newline
[deleted]: So what does the number 42 do for you? And what does pi do for you? Just curious.\newline
Sabakunoneji: 42 is a green and blue. I see multiple digit numbers as their individual colors side by side. Same with pi\newline
[deleted]: So when you see certain colors do you think of them mathematically?\colorbox{mediumgray}{\textup{[...]}}
\\\hline
\textbf{Relevant Document} \\\hline
Pi\_(disambiguation)\newline
Pi or $\pi$ is a mathematical constant equal to a circle's circumference divided by its diameter. Pi, $\pi$ or $\Pi$ may also refer to: Pi (letter), a Greek letter
\\\hline
\end{xltabular}
\end{center}

\subsubsection{QuanTemp}

\begin{center}\small
\begin{xltabular}{\textwidth}{|>{\itshape}X|}
\hline
\textbf{Instruction} \\\hline
Given a numerical claim, retrieve documents that can verify the claim.
\\\hline
\textbf{Query} \\\hline
Available COVID-19 vaccines are not linked to infertility or breast-feeding complications; 6,402 people did not die from the Moderna vaccine in February
\\\hline
\textbf{Relevant Document} \\\hline
Days after U.S. President Joe Biden said he would direct states to make all adults eligible for COVID-19 vaccines by May 1, a post on social media claimed that the vaccines cause infertility and that nursing mothers who have been vaccinated can cause harm to their babies. In addition, the post claims that over 6,000 people over the age of 50 died from the Moderna vaccine in February 2021. These claims are false. The main post in question, available \href{here}{here}, makes three main claims: 1) that the vaccine ``renders men and women sterile,'' 2) that ``if you are a nursing mother your baby can get serious side affects (sic)'' and 3) that ``6402 people over 50 died from the Moderna vaxx in February alone.'' Other social media posts making similar claims about vaccine-related infertility can be found \href{here}{here} and \href{here}{here}. At the time of this article's publication, over 115 million doses of the Pfizer-BioNTech, Moderna and Janssen vaccines, the three COVID-19 vaccines granted Emergency Use Authorization by the U.S. Food \& Drug Administration (FDA), have been administered in the United States according to the U.S. Centers for Disease Control and Prevention (CDC) (\href{here}{here}, \href{here}{here}). The Pfizer/BioNTech and Moderna vaccines use new messenger RNA (ribonucleic acid) technology to create an immune response and both require two shots. \colorbox{mediumgray}{\textup{[...]}}
\\\hline
\end{xltabular}
\end{center}

\subsubsection{WebTableSearch}

\begin{center}\small
\begin{xltabular}{\textwidth}{|>{\itshape}X|}
\hline
\textbf{Instruction} \\\hline
Given a question, retrieve relevant tabel to answer the question.
\\\hline
\textbf{Query} \\\hline
world interest rates table
\\\hline
\textbf{Relevant Document} \\\hline
Deposit interest rate (\%) | Data | Table\newline\newline
['Switzerland', 'Singapore', 'Hong\_Kong', 'Japan', 'Solomon\_Islands', 'Vanuatu', 'Papua\_New\_Guinea', 'Canada', 'Czech\_Republic', 'Bahrain', 'Algeria', 'Cambodia', 'Bhutan', 'Haiti', 'San\_Marino', 'China', 'Guyana', 'Nepal', \colorbox{mediumgray}{\textup{[...]}}, 'Zimbabwe', 'East\_Timor', 'Brunei', 'Slovakia', 'Kyrgyzstan', 'Laos', 'Syria', 'Faroe\_Islands'\newline\newline
2010-2014 2005-2009 2000-2004 1995-1999 1990-1994 1985-1989 1980-1984 Hide this Embed Metadata Graph Map Table View in WDI Tables World Development Indicators Catalog Sources International Monetary Fund, International Financial Statistics and data files. Deposit interest rate is the rate paid by commercial or similar banks for demand, time, or savings deposits. The terms and conditions attached to these rates differ by country, however, limiting their comparability. Deposit interest rate (\%)\newline\newline
Country name Switzerland Singapore Hong Kong SAR, China Japan Timor-Leste West Bank and Gaza Brunei Darussalam Solomon Islands Macao SAR, China Vanuatu Papua New Guinea Canada Czech Republic Bahrain Algeria Cambodia Bhutan Haiti San Marino China \colorbox{mediumgray}{\textup{[...]}}
\\\hline
\end{xltabular}
\end{center}

\subsubsection{FairRanking\_2021}

\begin{center}\small
\begin{xltabular}{\textwidth}{|>{\itshape}X|}
\hline
\textbf{Instruction} \\\hline
Given a description of a Wikiproject (title, keywords, and project scope), retrieve relevant documents from Wikipedia that are in need of editing to improve the quality of the documents. Ensure that documents that are about, or somehow represent, certain protected characteristics receive a fair exposure
\\\hline
\textbf{Query} \\\hline
Title: Agriculture\newline
Keywords: ['agriculture', 'crops', 'livestock', 'forests', 'farming']\newline
Scope: This WikiProject strives to develop and improve articles at Wikipedia related to crop production, livestock management, aquaculture, dairy farming and forest management. The project also covers related areas, including both governmental and NGO regulatory agencies, agribusiness, support agencies such as 4H, agricultural products including fertilizers and herbicides, pest management, veterinary medicine and farming equipment and facilities.
\\\hline
\textbf{Relevant Document} \\\hline
Abbreviation\newline\newline
manuscript text with scribal abbreviations An \textbf{abbreviation} (from Latin \textit{brevis}, meaning \textit{short}\text{} ) is a shortened form of a word or phrase, by any method. It may consist of a group of letters, or words taken from the full version of the word or phrase; for example, the word \textit{abbreviation} can itself be represented by the abbreviation \textit{abbr.}, \textit{abbrv.}, or \textit{abbrev.}; \textit{NPO}, for nil (or nothing) per (by) os (mouth) is an abbreviated medical instruction. It may also consist of initials only, a mixture of initials and words, or words or letters representing words in another language (for example, e.g., i.e. or RSVP). Some types of abbreviations are acronyms (which are pronounceable), initialisms (using initials only), or grammatical contractions or crasis. An abbreviation is a shortening by any of these, or other, methods. Acronyms, initialisms, contractions and crasis share some semantic and phonetic functions, and all four are connected by the term "abbreviation" in loose parlance.\text{name=harts} A contraction is a reduction of size by the drawing together of the parts; a contraction of a word or words is made by omitting certain letters or syllables and bringing together the first and last letters or elements, such as "I'm" . Thus contractions are a subset of abbreviations. Abbreviations have a long history, created so that spelling out a whole word could be avoided. This might be done to save time and space, and also to provide secrecy. In both Greece and Rome the reduction of words to single letters was common alse The British Cyclopaedia of the Arts, Sciences, History, Geography, Literature, Natural History, and Biography, Wm. S. Orr and Company, 1838, p.5. In Roman inscriptions, "Words were commonly abbreviated by using the initial letter or letters of words, and most inscriptions have at least one abbreviation". However, "some could have more than one meaning, depending on their context. (For example, can be an abbreviation for many words, such as , , , , , , and .) Handbook to Life in Ancient Rome], Infobase Publishing, 2004, p. 261. Abbreviations in English were frequently used from its earliest days. Manuscripts of copies of the old English poem \textit{Beowulf} used many abbreviations, for example the Tironian et () or for \textit{and}, and for \textit{since}, so that "not much space is wasted" Gelderen, E. v, A History of the English Language: Revised edition, John Benjamins Publishing Company, 2014, Ch. 4 1.] The standardisation of English in the 15th through 17th centuries included such a growth in the use of abbreviations.\colorbox{mediumgray}{\textup{[...]}}
\\\hline
\end{xltabular}
\end{center}

\subsubsection{FairRanking\_2022}

\begin{center}\small
\begin{xltabular}{\textwidth}{|>{\itshape}X|}
\hline
\textbf{Instruction} \\\hline
Given a description of a Wikiproject (title and keywords), retrieve relevant documents from Wikipedia that are in need of editing to improve the quality of the documents. Ensure that documents that are about, or somehow represent, certain protected characteristics receive a fair exposure.
\\\hline
\textbf{Query} \\\hline
Title: Architecture \newline
Keywords: ['museum', 'baroque', 'librarian', 'architecture', 'library', 'architect', 'cathedral', 'renaissance', 'decorative', 'regent', 'architectural', 'sculptor', 'catalogue', 'archive', 'monument', 'airport', 'skyscraper', 'heathrow', 'romanesque', 'island', 'cornish', 'arched', 'angeles', 'gothicmed', 'arch', 'designer', 'ornate', 'archcathedral', 'chancel', 'tidal', 'painter', 'masonry', 'basilica', 'sculpted', 'amphitheater', 'mount', 'spire', 'antiquity', 'sculpture', 'curatorial', 'boulevard', 'building', 'cottage', 'mansion', 'terrace', 'biographical', 'theatre', 'decorated', 'interlibrary', 'antique', 'exhibit', 'aquarium', 'monograph', 'city', 'historian', 'manor', 'harbour', 'exhibition', 'anthropology,urban,construction', 'heritage', 'pavilion', 'park']
\\\hline
\textbf{Relevant Document} \\\hline
Wright Creek (Nanticoke River tributary) \newline

Wright Creek is a long tributary to the Nanticoke River that rises in western Sussex County, Delaware. The creek straddles the Delaware state line for most of its course and is tidal for about half of its length. \newline

See also \newline
List of Delaware rivers \newline
List of rivers of Maryland \newline

References \newline
Rivers of Delaware \newline
Rivers of Maryland \newline
Rivers of Sussex County, Delaware \newline
Rivers of Caroline County, Maryland \newline
Tributaries of the Nanticoke River
\\\hline
\end{xltabular}
\end{center}

\subsubsection{NeuCLIR-Tech}

\begin{center}\small
\begin{xltabular}{\textwidth}{|>{\itshape}X|}
\hline
\textbf{Instruction} \\\hline
Articles describing the human reproductive system in biological terms from the perspective of a modern biologist are considered relevant. Articles describing the overall system such as a general description of the components or a lower level description such as specific cellular or molecular pathways involved in either the early development or adult stage maintenance of the systemo are relevant. Descriptions of mammalian reproductive system in general are considere somewhat valuable. Articles describing the reproductive system of a species outside of the class of mammalia are not relevant. Articles talking about human reproduction from other perspectives outside that of the biological sciences, such as from a historical or political perspective are not relevant.
\\\hline
\textbf{Query} \\\hline
human reproductive system
\\\hline
\textbf{Relevant Document} \\\hline
Research progress of SOX9 gene regulation of male mammalia reproductive activities\\

Sry-box contains protein 9 (SEX Determing Region Y-BOX 9, SOX9) gene is an important member of the sry-box containing protein (SRY-TYPE HMG BOX, SOX) gene family. Determing region of y Chromosome, sry) Another important gender decision gene after sry. Research in recent years shows that the SOX9 gene has played an important regulatory role in mammalian reproductive activities, and is closely different from gender differentiation, sperm and other reproductive activities. Related. This article mainly reviews the research progress of the mechanism of action during the embryo and post -lifting mammalian reproductive activities from the structural characteristics of the SOX9 gene. The mechanism and joint regulation mechanism with other genes provide a reference.\\

['mammal', 'Sry box contains protein 9 (SOX9)', 'Reproductive activity', 'Regulate']\\
Agriculture\\
Animal Husbandry and Veterinary Science
\\\hline
\end{xltabular}
\end{center}

\subsubsection{NeuCLIR\_2022}

\begin{center}\small
\begin{xltabular}{\textwidth}{|>{\itshape}X|}
\hline
\textbf{Instruction} \\\hline
Find reports on whether the star Betelgeuse going supernova will present a threat to the Earth. The red-giant star went through some dramatic changes in brightness at the end of 2019 before returning to its \"normal\" magnitude in 2020. Do not collect information on supernovae or stellar evolution in general. Only information specifically detailing the dangers from radiation and dust that Betelgeuse exploding would present to the Earth are required.
\\\hline
\textbf{Query} \\\hline
Danger of Betelgeuse going supernova
\\\hline
\textbf{Relevant Document} \\\hline
The probability of a dying star exploding greater than the Sun\newline\newline
Astronomers have recently announced that the star "El Joeza" or "Betelgeuse" of the constellation "Orion" is near the end of its life, and that its destruction will probably be accompanied by a major explosion.\newline
According to Isna and Cent, the second star in the constellation Orion is reportedly nearing the end of its life and will eventually end its life with a massive explosion called the supernova.\newline
The most massive stars in the world end their lives with a massive explosion called Supernova.\newline
A supernova occurs when a dying star begins to turn off.\newline
Then it explodes suddenly and produces a lot of light, leaving behind a small neutron nucleus.\newline
Pabat al-Jooza is a giant red star that is close to the end of its life, that is, at a time when the sun will reach it billions of years from now.\colorbox{mediumgray}{\textup{[...]}}
\\\hline
\end{xltabular}
\end{center}

\subsubsection{NeuCLIR\_2023}

\begin{center}\small
\begin{xltabular}{\textwidth}{|>{\itshape}X|}
\hline
\textbf{Instruction} \\\hline
We are Looking for articles that contain a case of financial corruption or bribery at institutional level. Cases of bribery in Olympics and sports federations are relevant. Cases of individuals\u2019 bribery are excluded. Investigating an institution to find out if they are involved in corruption will not be relevant. Ethical problems or sexual abuse are not relevant.
\\\hline
\textbf{Query} \\\hline
Corruption Bribery Sports Federation Olympics
\\\hline
\textbf{Relevant Document} \\\hline
Global weightlifting recklessness at risk of elimination of Olympic / Doubles and Disputes in the World Federation\newline\newline
With the rise of disputes in the World Federation of Weightlifting, IOC ’ s warning seems not to be taken seriously and now threatens the risk of elimination from the Olympics more than ever before.\newline
According to ISNA, the head of the World Federation of Weightlifting has put the field at risk of elimination from the Olympics, and even Thomas Bach, the chairman of the International Olympic Committee, expressed concern about the situation of the field, and the current situation threatens the position of weightlifting in the 2024 Olympics.\newline
* The beginning of the events in weightlifting of a documentary began.\newline
A few months ago, a German network broadcast a documentary in which it unveiled the existence of corruption and systematic doping in the World Federation of Weightlifting.\newline
At that time Tamash Ayan was the president.\newline
This caused a lot of noise and led the Executive Board of the Federation to decide to suspend Ayan in order to conduct investigations on charges.\colorbox{mediumgray}{\textup{[...]}}
\\\hline
\end{xltabular}
\end{center}

\subsubsection{ProductSearch\_2023}

\begin{center}\small
\begin{xltabular}{\textwidth}{|>{\itshape}X|}
\hline
\textbf{Instruction} \\\hline
Given a search query, retrieve products that are relevant to the query.
\\\hline
\textbf{Query} \\\hline
HAPY SHOP 80 Pcs Silver Alligator Hair
\\\hline
\textbf{Relevant Document} \\\hline
Product Description HAPY SHOP 80 Pcs Silver Alligator Hair Clip Flat Top with Teeth 3 inch and 1.6 inch for Hair Care, Arts \& Crafts Projects, Dry Hanging Clothing,2 Size 80 pack Silver Alligator Hair Clips in 2 size, big size can provides strength and ample capacity for salon hair spraying,small size can deal with the details. Read more Aligned with teeth style closure,so items they hold will not slip but not so tight that they can cause damage. Read more Size 40 x 3 inch hair clips 40 x 1.6 inch clips Material Made of nickel plated metal with smooth surface,can greatly handle thick or thin hair. Durable Durable for long term application. Read more Read more
\\\hline
\end{xltabular}
\end{center}

\subsubsection{ToT\_2023}

\begin{center}\small
\begin{xltabular}{\textwidth}{|>{\itshape}X|}
\hline
\textbf{Instruction} \\\hline
You are an expert in movies, assisting someone in recalling the name of a movie that's on the tip of their tongue. For the given tip-of-the-tongue information requests, retrieve Wikipedia pages of potential movie titles that match the description provided.
\\\hline
\textbf{Query} \\\hline
Title: Girl in a red dress enters a bizarre shop, where she gets chloroformed by the weird owner\newline
This was a short movie I saw either on YT or Vimeo, not sure. Cannot find it now for the love of\u2026 A girl in a red dress enters a bizarre shop, to buy a present for her boyfriend (she says so), goes downstairs and inspects a shelf full of strange artifacts, when the shop owner chloroforms her and chains her. She wakes up and finds a way to cut herself loose, but she doesn't fight the owner, who chains her again and makes her get dressed in a pink ball dress. That's pretty much it ? Thanks.
\\\hline
\textbf{Relevant Document} \\\hline
The Collector (1965 film)\\
\\
The Collector is a 1965 psychological horror film directed by William Wyler and starring Terence Stamp and Samantha Eggar. Its plot follows a young Englishman who stalks a beautiful art student before abducting and holding her captive in the basement of his rural farmhouse. It is based on the 1963 novel of the same title by John Fowles, with the screenplay adapted by Stanley Mann and John Kohn. Wyler turned down ``The Sound of Music'' to direct the film.\\
Most of the film was shot on soundstages in Los Angeles, though exterior sequences were filmed on location in London, Forest Row in East Sussex and Westerham in Kent. Filming occurred in the late spring and early summer of 1964. Wyler's original cut ran approximately three hours but was trimmed to two hours at the insistence of the studio and producer.\\
``The Collector'' premiered at the Cannes Film Festival in May 1965, where both Stamp and Eggar won the awards for Best Actor and Best Actress, respectively. Upon its theatrical release in June 1965, the film received largely favourable reviews. Eggar won a Golden Globe Award for Best Actress in a Motion Picture – Drama for her performance, and was also nominated for the Academy Award for Best Actress, while Wyler received a nomination for Best Director. It was the last of Wyler's record 12 Academy Award nominations for Best Director.\\
\\
Plot.\\
Freddie is a lonely, socially-awkward young man who purchases a farmhouse with winnings he has earned from the football pools. An amateur entomologist, he spends his time capturing butterflies, of which he has a large collection. Frederick begins stalking a bourgeois London art student named Miranda Grey. One day, Frederick follows Miranda into a pub in Hampstead before abducting her on the street, incapacitating her with chloroform. \colorbox{mediumgray}{\textup{[...]}}
\\\hline
\end{xltabular}
\end{center}

\subsubsection{ToT\_2024}

\begin{center}\small
\begin{xltabular}{\textwidth}{|>{\itshape}X|}
\hline
\textbf{Instruction} \\\hline
You are an expert in movies, landmarks, and celebrities. You are helping someone recall the name of a movie, landmark, or celebrity that's on the tip of their tongue. For these tip-of-the-tongue information requests, retrieve Wikipedia pages of potential matches for the movie, landmark, or celebrity being described.
\\\hline
\textbf{Query} \\\hline
Man trapped by a mother and her daughter .\newline
A man is trapped in a flat by a mother and her daughter. I remember little else about this movie, except that it was foreign, possibly Italian, dubbed into English.
\\\hline
\textbf{Relevant Document} \\\hline
The Trap (1985 film)\newline\newline
The Trap (), also known as Collector's Item, Dead Fright and The Cage, is a 1985 erotic thriller directed by Giuseppe Patroni Griffi (his last theatrical film), and starring Tony Musante, Laura Antonelli, and Florinda Bolkan. Famed Italian horror director Lucio Fulci contributed to the screenplay (this film was done during the time Fulci was recovering from hepatitus, so he was unable to direct it).\newline
The film is based on a story called "L'Occhio", written by filmmaker Francesco Barilli. Barilli intended to make the film himself, but had trouble securing backing and balked at the producers wanting Shelley Winters in the lead role. So he sold the idea to Griffi and let him produce and direct it, retitling it "The Trap". Barilli said of the finished product "Lets' talk frankly here, that movie sucks..." and Fulci even used profanity alluding to his opinion of Griffi, who he felt stole his chance to direct the film. \newline\newline
Plot.\newline
Michael Parker is a successful American businessman living in Italy with his girlfriend Hélène. However, when she leaves on vacation, Michael soon becomes involved in an affair with Marie, a woman he once had a one-night stand with. This affair proves more difficult for Michael, as Marie is not going to let him off the hook again so easily. To complicate matters worse, Marie's young daughter Jacqueline also finds herself attracted to Michael, resulting in an incestuous love triangle.
\\\hline
\end{xltabular}
\end{center}

\subsubsection{ExcluIR}

\begin{center}\small
\begin{xltabular}{\textwidth}{|>{\itshape}X|}
\hline
\textbf{Instruction} \\\hline
Given a search query, retrieve relevant passages. Ensure not to retrieve excluded passages described in the query.
\\\hline
\textbf{Query} \\\hline
Excluding Fatal Instinct, which is a 1993 American erotic thriller comedy film directed by Carl Reiner, in which other movies did the American actress Mary Sean Young portray characters?
\\\hline
\textbf{Relevant Document} \\\hline
Sean Young\newline
Mary Sean Young (born November 20, 1959) is an American actress. She is best known for her performances in the films ``Blade Runner'' (1982), ``Dune'' (1984), ``No Way Out'' (1987), ``Wall Street'' (1987), ``Cousins'' (1989) and ``'' (1994).
\\\hline
\end{xltabular}
\end{center}

\subsubsection{FollowIR\_Core17}

\begin{center}\small
\begin{xltabular}{\textwidth}{|>{\itshape}X|}
\hline
\textbf{Instruction} \\\hline
Find a study or article that addresses this question.\newline
Persons living near radio towers and more recently persons using car (mobile) phones have been diagnosed with brain cancer. The argument rages regarding the direct association of one with the other. The incidence of cancer among the groups cited is considered, by some, to be higher than that found in the normal population. A relevant document includes any experiment with animals, statistical study, articles, news items which report on the incidence of brain cancer being higher/lower/same as those persons who live near a radio tower and those using car (mobile) phones as compared to those in the general population. Any mentions of leukemia is not relevant.
\\\hline
\textbf{Query} \\\hline
Evidence that radio waves from radio towers or car (mobile) phones affect brain cancer occurrence.
\\\hline
\textbf{Relevant Document} \\\hline
Brain Tumors: Elusive, Varied and Not Always Deadly\newline
elsewhere in the body -- although, as in Kathleen's case, the primary cancer is sometimes not detected until after the metastatic brain tumor has been found. Lung, breast and colon cancers, as well as melanomas, often spread to the brain. There has been much speculation about the possible causes of brain cancers, and especially their apparent increase. About 5 percent are hereditary. Among suggested environmental factors are low-energy electromagnetic fields from objects like cellular phones, power lines and household appliances, although considerable research into the matter has yet to yield any definitive evidence of such a risk. To be sure, high-dose radiation delivered to the head, including therapy for brain tumors, can increase the risk of brain cancer. There is no link, however, to low-dose radiation delivered through diagnostic X-rays or workplace exposure to ionizing radiation. \colorbox{mediumgray}{\textup{[...]}}
\\\hline
\end{xltabular}
\end{center}

\subsubsection{FollowIR\_News21}

\begin{center}\small
\begin{xltabular}{\textwidth}{|>{\itshape}X|}
\hline
\textbf{Instruction} \\\hline
Find authoritative sources to answer this health-related question.\newline
China recently discovered a new coronavirus strain that is similar to MERS.  Tell me about the symptoms of MERS, the incubation period for infection, and the lethality rate.  Information on vaccines and treatments is relevant.  Official sources of information on MERS also is relevant.  Information on the origins of MERS is not relevant nor are the specific locations of previous outbreaks.  Editorials are not relevant. If the document discusses a potential animal origin, please ignore the document.
\\\hline
\textbf{Query} \\\hline
What is the Middle East Respiratory Syndrome (MERS)?
\\\hline
\textbf{Relevant Document} \\\hline
World digest: June 13, 2015 \\
The World Health Organization says South Korea's outbreak of Middle East Respiratory Syndrome (MERS) was ``large and complex'' and more cases should be anticipated. SOUTH KOREA Emergency meeting on MERS outbreak The World Health Organization said Saturday that it would hold an emergency meeting on Tuesday to consider South Korea's outbreak of Middle East Respiratory Syndrome (MERS), which it described as ``large and complex.'' The virus has infected 138 people in South Korea and killed 14 of them since it was first diagnosed May 20 in a businessman who had returned from a trip to the Middle East. The U.N. health agency said that more cases should be anticipated but that the disease was confined to hospitals, with no sign it was spreading in the community. There was also no indication that the MERS virus in South Korea had changed to become more transmissible, said Keiji Fukuda, the agency's assistant director general, at a news conference at the Health Ministry in Sejong, south of the capital, Seoul. The meeting Tuesday of the MERS emergency committee, which comprises international health experts from WHO member states, will provide technical updates on epidemiology as well as advice on future actions to be taken, the agency said. --- Reuters IRAN Nuclear deal is ``within reach'' President Hassan Rouhani said a final nuclear deal is ``within reach'' as Iran and six world powers face a June 30 deadline for an agreement. The country has taken emergency measures to stop the spread of Middle East Respiratory Syndrome. \colorbox{mediumgray}{\textup{[...]}}
\\\hline
\end{xltabular}
\end{center}

\subsubsection{FollowIR\_Robust04}

\begin{center}\small
\begin{xltabular}{\textwidth}{|>{\itshape}X|}
\hline
\textbf{Instruction} \\\hline
Find a document comparing vehicle crashworthiness relevant to this question.\newline
A relevant document will contain information on the  crashworthiness of a given vehicle or vehicles that  can be used to draw a comparison with other vehicles.   The document will have to describe/compare vehicles,  not drivers.  For instance, it should be expected  that vehicles preferred by 16-25 year-olds would be  involved in more crashes, because that age group is involved in more crashes.  I would view number of  fatalities per 100 crashes to be more revealing of  a vehicle's crashworthiness than the number of crashes per 100,000 miles, for example. You should ignore any recall related articles, as that means they will be fixed, and exclude any anecdotal information of individual crashes.
\\\hline
\textbf{Query} \\\hline
Which are the most crashworthy, and least crashworthy,  passenger vehicles?
\\\hline
\textbf{Relevant Document} \\\hline
FT 25 JUN 92 / Executive Cars (21): Two litres is quite enough - Unless status means more than a combination of performance and reasonable economy, there is every incentive to go for a modern, high-efficiency 2-litre engine. Stuart Marshall assesses the latest range of vehicles and finds an embarrassment of choice \newline How They Go\newline to sell in Britain for a similar figure with a 2-litre engine and automatic transmission when it arrives in early autumn. Safrane majors on ride quality and silence. The Mercedes-Benz 190E with 1.8-litre or 2-litre engines, now nearly 10 years old and due soon for replacement, is unmatched in its price class for status and sheer merit. Its bank-vault build quality and conservative styling pay off in high retained values. The pleasure of driving one is to be equated with the feeling one gets when upgraded to first from business class. The Peugeot 605 SLi 2.0, steel sprung but otherwise similar mechanically to a Citroen XM, is a roomy, quiet and undemanding drive. Rover's 820, restyled and improved within the past year, has build quality to match that of any European rival and is a driver's car which passengers enjoy equally. Volvo's five-cylinder, front wheel-driven 850GLT is an outstanding newcomer. It may look rather like a mid-1980s rear drive Volvo, but everything about it is original - except, that is, the styling. Performance is lively, the ride is good, the handling supremely safe and, should the worst happen, its crash survivability is probably unmatched. A feature of the past year has been the \colorbox{mediumgray}{\textup{[...]}}
\\\hline
\end{xltabular}
\end{center}

\subsubsection{InstructIR}

\begin{center}\small
\begin{xltabular}{\textwidth}{|>{\itshape}X|}
\hline
\textbf{Instruction} \\\hline
I am a DIY enthusiast looking to upcycle a dresser. I aim to find creative ideas and sustainability-focused blogs that explain the various ways a dresser drawer can be repurposed or refurbished, thereby enhancing my project with unique and eco-friendly approaches. [SEP] what is a dresser drawer
\\\hline
\textbf{Query} \\\hline
what is a dresser drawer
\\\hline
\textbf{Relevant Document} \\\hline
A chest of drawers, alternatively known in certain regions as a bureau, stands as a versatile furniture item characterized by several parallel drawers that are placed in a stacked alignment vertically. Typically, this household item reaches around waist height and is often accompanied by a space to accommodate a reflective surface. Enthusiasts of the `do it yourself' approach frequently direct their inventive energy toward transforming these drawers into distinctively eco-conscious home additions. Whether through imaginative restorations or novel adaptations, such elements of home decor can be elevated to function beyond their traditional, storage-centric roles.
\\\hline
\end{xltabular}
\end{center}

\subsubsection{NevIR}

\begin{center}\small
\begin{xltabular}{\textwidth}{|>{\itshape}X|}
\hline
\textbf{Instruction} \\\hline
Given a search query, retrieve relevant passages. Pay special attention to any negation in the query and the passages, as this can make seemingly relevant passages irrelevant.
\\\hline
\textbf{Query} \\\hline
What occupied islands id the Portuguese colonize and develop?
\\\hline
\textbf{Relevant Document} \\\hline
Before the arrival of the Europeans, the African slave trade, centuries old in Africa, was not yet the major feature of the coastal economy of Guinea. The expansion of trade occurs after the Portuguese reach this region in 1446, bringing great wealth to several local slave trading tribes. The Portuguese used slave labour to colonize and develop the Cape Verde islands where they founded settlements and grew cotton and indigo shortly after the Portuguese cleared out the remaining indigenous inhabitants. They then traded these goods, in the estuary of the Geba River, for black slaves captured by other black peoples in local African wars and raids.
\\\hline
\end{xltabular}
\end{center}

\subsubsection{IFEval}

\begin{center}\small
\begin{xltabular}{\textwidth}{|>{\itshape}X|}
\hline
\textbf{Instruction} \\\hline
Retrieve responses to the given question. It is crucial that the responses strictly follow to the specified instruction: \textbf{In your response, the word constable should appear at least 2 times.}. Any response that does not fully comply with this instruction should be considered irrelevant.
\\\hline
\textbf{Query} \\\hline
What happened in 719, when the Tang dynasty was in power?
\\\hline
\textbf{Relevant Document} \\\hline
In 719, during the Tang dynasty's rule, there were significant reforms implemented in the local administration. The role of constables was strengthened, and they were tasked with maintaining law and order in their respective districts. Constables were also provided with better training and resources to improve their effectiveness in policing the communities they served. These changes led to a more efficient and organized system of law enforcement, contributing to greater stability and security within the empire.
\\\hline
\textbf{Irrelevant Document} \\\hline
In 719, during the Tang dynasty in China, a major rebellion known as the An Lushan Rebellion broke out. The rebellion was led by the general An Lushan, who rebelled against the Tang government, leading to a destructive civil war that lasted for several years. The rebellion caused widespread chaos and devastation throughout the empire, leading to a significant loss of life and a weakening of the Tang dynasty's power. It had a long-lasting impact on the stability of the dynasty and the social and economic structures of the time.
\\\hline
\end{xltabular}
\end{center}

\begin{center}\small
\begin{xltabular}{\textwidth}{|>{\itshape}X|}
\hline
\textbf{Instruction} \\\hline
Retrieve responses to the given question. It is crucial that the responses strictly follow to the specified instruction: \textbf{Entire output should be wrapped in JSON format. You can use markdown ticks such as ```.}. Any response that does not fully comply with this instruction should be considered irrelevant.
\\\hline
\textbf{Query} \\\hline
What is the history of NYC prospect park?
\\\hline
\textbf{Relevant Document} \\\hline
\texttt{\{} \newline
  \hspace*{2em} \texttt{"NYC Prospect Park": \{} \newline
  \hspace*{4em} \texttt{"History": "Prospect Park is a public park in the borough of Brooklyn in New York City. It was designed by Frederick Law Olmsted and Calvert Vaux, who also designed Central Park. Construction of Prospect Park began in 1866 and was completed in 1873. The park was designated a National Historic Landmark in 1962. It is known for its naturalistic design, featuring large expanses of grass, woodlands, and bodies of water, as well as various recreational facilities for visitors."}, \newline
  \hspace*{4em} \texttt{"Key Features": ["Long Meadow", "Prospect Park Lake", "Brooklyn Botanic Garden", "Brooklyn Museum", "LeFrak Center at Lakeside"]}, \newline
  \hspace*{4em} \texttt{"Events": ["Concerts", "Outdoor Movies", "Running Races", "Festivals"]} \newline
  \hspace*{2em} \texttt{\}} \newline
  \texttt{\}} \newline
\\\hline
\textbf{Irrelevant Document} \\\hline
Prospect Park is a 526-acre public park in Brooklyn, New York City. It was designed by Frederick Law Olmsted and Calvert Vaux, who also designed Central Park in Manhattan. Prospect Park was created in the 19th century as part of the overall urban planning and development of Brooklyn.\newline

The park was officially opened to the public in 1867, although construction continued for several more years. Prospect Park was intended to provide an oasis of nature and recreation for the residents of Brooklyn, as well as to serve as a counterpart to Manhattan's Central Park.\newline

Over the years, Prospect Park has been a popular destination for both locals and tourists, offering a wide range of activities and amenities, including playgrounds, sports fields, a zoo, and an outdoor concert venue. The park is also home to various historical landmarks, such as the Boathouse and the Lefferts Historic House.\newline

Today, Prospect Park remains one of the most beloved and iconic green spaces in New York City, attracting millions of visitors each year.
\\\hline
\end{xltabular}
\end{center}

\begin{center}\small
\begin{xltabular}{\textwidth}{|>{\itshape}X|}
\hline
\textbf{Instruction} \\\hline
Retrieve responses to the given question. It is crucial that the responses strictly follow to the specified instruction: \textbf{In your entire response, refrain from the use of any commas.}. Any response that does not fully comply with this instruction should be considered irrelevant.
\\\hline
\textbf{Query} \\\hline
I am planning a trip to Japan, and I would like thee to write an itinerary for my journey in a Shakespearean style.
\\\hline
\textbf{Relevant Document} \\\hline
Day One: Upon the dawn of thine arrival in fair Nippon thou shalt traverse to the city of Tokyo flourishing with lights and marvels aplenty thine eyes shall feast upon the grand imperial gardens and thou shalt bask in the serenity of Meiji Shrine \newline \newline
Day Two: Thenceforth to Kyoto go thou and witness the splendid temples of Kinkaku-ji and Fushimi Inari-taisha where the spirits of old still whisper unto the winds and the cherry blossoms doth sway in gentle rhythm \newline \newline
Day Three: On the third morrow quench thy thirst for ancient tales in the city of Nara where sacred deer roam and the great Buddha in Todai-ji's embrace doth lie in wait \newline \newline
Day Four: A journey to the highlands of Hakone undertake thou then bathe in the onsen where the waters warm doth soothe the weary soul and gaze upon Mount Fuji whose peak doth pierce the heavens \newline \newline
Day Five: Return to the bustling heart of Tokyo and revel in the artistry of Akihabara's wonders and Shibuya's boundless sea of life ere thou takest leave and bid adieu to the land of the rising sun thus concluding thine enchanting sojourn
\\\hline
\textbf{Irrelevant Document} \\\hline
Day 1:\newline
Hark! Upon yon rising sun, alight in Tokyo, the city divine,\newline
Where towers reach thither, and lights doth entwine.\newline
Shall visit Asakusa, sacred and old,\newline
The Senso-ji Temple, with splendour to behold.\newline
\newline
Day 2:\newline
To Kyoto hie, by swift bullet train,\newline
Where ancient temples and gardens remain.\newline
The Fushimi Inari, with torii gates bright,\newline
A thousand fold crimson, they maketh a sight.\newline
\newline
Day 3:\newline
In Arashiyama, ‘neath bamboo so tall,\newline
Stroll through groves where shadows doth fall.\newline
The monkeys at Iwatayama, lively and free,\newline
In their mountain abode, full of glee.\newline
\newline
Day 4:\newline
To Nara venture, and their sacred deer,\newline
Roam 'mid pagodas, Earth's wonders appear.\newline
Todaiji Temple, with Buddha so grand,\newline
In a park where quietude doth stand.\newline
\newline
Day 5:\newline
Osaka calls, metropolis with zeal,\newline
Where food and commerce together doth reel.\newline
Harbor to Dotonbori, with lights all a-glare,\newline
Takoyaki and sights beyond all compare.\colorbox{mediumgray}{\textup{[...]}}
\\\hline
\end{xltabular}
\end{center}
\colorbox{mediumgray}{\textup{[...]}}

\begin{center}\small
\begin{xltabular}{\textwidth}{|>{\itshape}X|}
\hline
\textbf{Instruction} \\\hline

\\\hline
\textbf{Query} \\\hline

\\\hline
\textbf{Relevant Document} \\\hline

\\\hline
\end{xltabular}
\end{center}

\subsection{TREC}\label{TREC}

\subsubsection{TREC Clinical Decision Support Track 2014} \label{cds14}

% In this track, the participants should answer common clinical questions by retrieving biomedical articles.
% The questions are usually related to diagnosis, testing, treatment, etc.
% The biomedical articles here are all short case reports of patients instead of using actual full-text medical records:
This track studied the literature retrieval task in clinical decision support systems. It used case reports as queries to retrieve relevant biomedical articles.

\begin{itemize}
\item The queries are case reports describing the patient's symptoms, medical history, etc., but omitting information about diagnosis, tests, or treatment. For example, "A 58-year-old African-American woman with hypertension and obesity presents with exercise-related episodic chest pain radiating to the back."

\item The target document collection is an open-access subset of PubMed Central (PMC), an online repository of freely available full-text biomedical literature. Specifically, a snapshot of the PMC open access subset taken on January 21, 2014, is used, containing a total of 733,138 articles. 

\item Relevance is judged based on whether the document provided useful information of the specified clinical information type (diagnosis, test, or treatment) for the given case report. The relevance is divided into 3 levels: 
\begin{itemize}
    \item Definitely relevant(2): The document provided information of the specified type (diagnosis, test, treatment) and is relevant to the particular patient case described in the topic.
    \item Possibly relevant(1): The document is not immediately informative on its own, but may be relevant in the context of a broader literature review.
    \item Not relevant(0): The document either did not provide information of the specified type or is not applicable to the patient's case.
\end{itemize}

\item We annotate instructions like this: "Given a medical case record that consists of a summary and a full description, retrieve biomedical articles from PubMed Central that provide useful information for answering the following clinical question: What is the patient's diagnosis? / What tests should the patients receive? / How should the patient be treated?"

\item The following is an example:
[A table]
\end{itemize}

\subsubsection{TREC Clinical Decision Support Track 2015}
The same as \ref{cds14}
\subsubsection{TREC Clinical Decision Support Track 2016}
The same as \ref{cds14}
% \subsubsection{TREC Precision Medicine Track 2017}
% The 2017-2019 Precision Medicine Track aims to assist in the treatment of cancer patients by providing precision medicine-related information. Using synthetic cases created by the MD Anderson Cancer Center, participants are challenged to retrieve relevant clinical trials.
% \begin{itemize}
% \item Queries in this task are synthetic patient cases created by MD Anderson precision oncologists

% \item Documents in this task are clinical trials

% \item The relevance is judged by four topic dimensions (disease, gene, demographic, and other). Each of these corresponds to 3-4 categories (e.g., a disease can be an "exact", "more general", "more specific", or "not disease" match).

% \item We annotate instructions like this

% \item The following is an example:
% [A table]
% \end{itemize}
\subsubsection{TREC Clinical Trials Track 2021} \label{ctt21}
This track studies the task of retrieving clinical trials. It uses simulated patient case descriptions from electronic health records as queries to retrieve clinical trial descriptions published on ClinicalTrials.gov.
\begin{itemize}
\item The queries in the TREC 2022 Clinical Trials Track are brief patient case descriptions resembling admission notes, including details like age, medical history, symptoms, and test results. Each multi-sentence paragraph or list describes a realistic patient case derived with a specific disease in mind, but without revealing the disease. The 50 topics serve as queries to retrieve relevant clinical trials based on whether the described patient meets the trial's eligibility criteria.

\item The document collection is a snapshot from April 27, 2021, of all clinical trials available on ClinicalTrials.gov, which contained 375,581 trial descriptions. Each trial is identified by its National Clinical Trial (NCT) number, which serves as the document ID. The core part of each trial description relevant for matching to patient cases is the eligibility criteria section, which lists the inclusion and exclusion criteria that determine if a patient qualifies for the trial or not.

\item Relevance is determined based on whether the patient meets the inclusion criteria and exclusion criteria for the trial. The relevance judgments in this task are divided into 3 levels:
\begin{itemize}
    \item Eligible(2): The patient case description meets all the inclusion criteria for the clinical trial and does not violate any exclusion criteria. The patient would be eligible to enroll in the trial.
    \item Excluded(1): The patient has the condition that the trial is targeting, but violates one or more of the exclusion criteria, making them ineligible for the trial.
    \item Not Relevant(0): The patient case description does not contain enough information to determine eligibility, or clearly does not match the trial's criteria. The patient is simply not relevant for that particular trial.
\end{itemize}

\item We annotate instructions like this: "Given a patient health record, retrieve clinical trials that are suitable for that patient. Rials are 'relevant' if the patient met the inclusion criteria and did not meet any exclusion criteria; Rials are 'partially relevant' if the patient met the inclusion criteria but is excluded by one or more exclusion criteria."

\item The following is an example:
[A table]
\end{itemize}
\subsubsection{TREC Clinical Trials Track 2022}
The same as \ref{ctt21}.
\subsubsection{TREC Clinical Trials Track 2023}
The same as \ref{ctt21}, but the documents are updated to 2023.

\subsubsection{TREC Conversational Assistance Track 2019}
Similar to \ref{cat22}, The document collection is compiled from the following sources:

MS MARCO Passage Ranking collection

TREC CAR paragraph collection v2.0

\subsubsection{TREC Conversational Assistance Track 2020}
Similar to \ref{cat22}, The document collection is compiled from the following sources:

MS MARCO Passage Ranking collection

TREC CAR paragraph collection v2.0
\subsubsection{TREC Conversational Assistance Track 2021}
Similar to \ref{cat22}, The document collection is compiled from the following sources:

KILT Wikipedia 

MS MARCO (Documents) 

\subsubsection{TREC Conversational Assistance Track 2022} \label{cat22}
This track studies the Conversational Passage Retrieval (ConvPR) task. The system needs to retrieve relevant document passages based on the user's query and previous conversational context and generate natural language responses.

\begin{itemize}
\item The queries are formed by the user's natural language utterances, containing their information needs. The utterances evolve and change as the conversation progresses, reflecting the dynamic nature of the user's information needs.
\item The document collection includes documents from MS MARCO V2 and Wikipedia articles from the KILT dump. Each document is split into canonical passages of up to 250 words. The collection contains around 17 million passages in total.

\item The relevance judgments are based on whether the passage contains useful information to satisfy the user's current utterance. The relevance levels are as follows:
\begin{itemize}
    \item Not Relevant(0): The passage does not relate to the current conversational context at all.
    \item Partially Relevant(1): The passage is somewhat related to the conversational context, but the relevance is marginal or too tangential.
    \item Relevant(2): The passage is relevant to the conversational context, but it is not entirely clear why this particular passage is retrieved.
    \item Highly Relevant(3): The passage directly follows from and relates to the conversational context, and it is clear why this passage is retrieved.
    \item Perfect Match(4): The passage perfectly matches the information need expressing in the conversational context.
\end{itemize}

\item We annotate instructions like this: "Given a dialogue history, retrieve passages to answer the user's question in the last turn."

\item The following is an example:
[A table]
\end{itemize}

\subsubsection{TREC Dynamic Domain Track 2015}  \label{dd15}
This track studies dynamic, exploratory search tasks, simulating the interaction between professional searchers and search systems. It uses 2-4 word phrases as initial queries to retrieve documents from specific domain collections.
\begin{itemize}
\item The initial query is a 2-4 word phrase representing a topic, and the system needs to retrieve relevant documents for that topic.

\item The documents are from three domains: Ebola, Illicit Goods, and Local Politics. They include web pages, PDF files, and tweets. The data sources include government agencies, news organizations, social media, etc.

\item Relevance is determined based on how well the text passages from documents are associated with the subtopics of the main topic. The relevance is divided into 4 levels:
\begin{itemize}
    \item Marginally relevant(1): A passage judged as marginally relevant means it is only slightly or peripherally related to the subtopic. It may contain some tangentially relevant information but does not directly address the core aspects of that subtopic.
    \item Relevant(2): A relevant passage means the content is definitely relevant and on-topic for that particular subtopic. It contains useful information that helps satisfy and answer aspects of the information need represented by that subtopic.
    \item Highly relevant(3): A highly relevant passage is one that is extremely important and central to fully covering and addressing that subtopic. It likely contains key details, facts, or analysis that are critical for comprehensively answering the subtopic.
    \item Key results(4): Passages judged as key results are the most essential and vital pieces of information required to satisfy that subtopic completely. These are the critical passages without which the subtopic cannot be fully answered or resolved satisfactorily.
\end{itemize}

\item We annotate instructions like this "Given a domain and a topic associated with multiple sub-topics, the goal is to find passages relevant to all sub-topics. The feedback field includes the retrieved passages from an initial system, along with the sub-topics and their corresponding relevance scores. Your task is to retrieve passages related to the sub-topics that are not retrieved by the initial system. Ensure that you exclude any passages already retrieved by the initial system."

\item The following is an example:
[A table]
\end{itemize}
\subsubsection{TREC Dynamic Domain Track 2016}
The same as \ref{dd15}
\subsubsection{TREC Dynamic Domain Track 2017}
The same as \ref{dd15}, but the documents are updated to the New York Times.
\subsubsection{TREC Fair Ranking Track 2019} \label{fr19}
This track studied the fair ranking retrieval task. It used queries from the academic search engine Semantic Scholar to re-rank academic paper abstracts.
\begin{itemize}
\item The query data came from the query logs of Semantic Scholar, containing the query string, displayed documents, and number of clicks for each document. After filtering and sampling, 652 training queries and 635 evaluation queries are provided.

\item The documents are academic paper abstracts from Semantic Scholar, including paper ID, DOI, title, abstract, author IDs, and citation information. The document data came from the Semantic Scholar Open Corpus provided by the Allen Institute for Artificial Intelligence.

\item Relevance is determined based on whether a document had at least one click in the query logs. If it had a click, it is considered relevant(1), otherwise non-relevant(0).

\item We annotate instructions like this "Given a query, retrieve relevant academic articles. Ensure fair exposure to different groups of authors, where the group definitions could based on demographics, stature, topic, and others."

\item The following is an example:
[A table]
\end{itemize}
\subsubsection{TREC Fair Ranking Track 2020}
Similar to \ref{fr19}, only the query and corpus are updated
\subsubsection{TREC Fair Ranking Track 2021}
Similar to \ref{fr19}, only the query and corpus are updated
\subsubsection{TREC Genomics Track 2004}
This track aims to improve information retrieval in the biomedical field, with participants developing algorithms to search 160,000 full-text articles from 59 journals based on real biologists' questions. 
The 2004 Genomics Track included two tasks: an ad hoc retrieval task, which involved searching the MEDLINE database based on real biologists' information needs, and a full-text document categorization task, which simulated the curation process of the Mouse Genome Informatics system.
In this paper, we only use data from ad-hoc tasks. Because classification tasks are not conducive to the construction of retrieval benchmarks
\paragraph{ad hoc retrieval task} \label{genoadhoc}
The ad hoc retrieval task mimics a situation where a biomedical researcher has an information need and searches a document collection (the MEDLINE subset) to find relevant medical documents.
\begin{itemize}
\item The queries originated from interviews with 43 biologists, yielding 74 initial information needs. These needs are reviewed and modified to create 50 final query topics. Each query topic contained fields like a title, statement of the information need, and background context.

\item The document collection is a 10-year subset of the MEDLINE bibliographic database maintained by the U.S. National Library of Medicine, containing a large amount of literature related to genomics.

\item The relevance is divided into 3 levels.

\begin{itemize}
    \item Definitely Relevant (2):
    The document is a clear, definite match for the information need expressed in the topic description.
    The content of the document directly and completely addresses the stated information need.
    \item Possibly Relevant (1):
    The document appears related and potentially relevant to the information needed, but its relevance is not definite.
    The document may partially address the information needed or address it in a tangential way.
    There is some uncertainty about whether the document truly satisfies the stated information need.
    \item Not Relevant (0):
    The document does not appear to be relevant or address the stated information need at all.
    There is no meaningful relationship between the document's content and what the topic is asking for.
\end{itemize}

\item We annotate instructions like this "Given a biomedical question, retrieve documents from the MEDLINE bibliographic database to answer the question. The following is the context of this search: Ferroportin1 (also known as SLC40A1; Ferroportin 1; FPN1; HFE4; IREG1; Iron regulated gene 1; Iron-regulated transporter 1; MTP1; SLC11A3; and Solute carrier family 11 (proton-coupled divalent metal ion transporters), member 3) may play a role in iron transport."

\item The following is an example:
[A table]
\end{itemize}
\subsubsection{TREC Genomics Track 2005}
The same as \ref{genoadhoc}
\subsubsection{TREC Genomics Track 2006}
The same as \ref{genoadhoc}
\subsubsection{TREC Genomics Track 2007}
The same as \ref{genoadhoc}
\subsubsection{TREC Legal Track 2010} \label{legal10}
This Track simulates the actual conditions of document review in civil litigation, aiming to find documents responsive to production requests.
\begin{itemize}
\item The queries are modeled on requests for production in civil litigation, specifying categories of documents that must be identified. Each request for production corresponds to a topic.
There are 4 queries total - 3 subject-matter queries (301-303) and 1 privilege query (304) focused on identifying privileged documents.

Query 301 - Documents related to onshore or offshore oil and gas drilling or extraction activities.

Query 302 - Documents related to responses to oil and gas spills, blowouts, releases, or pipeline eruptions.

Query 303 - Documents related to lobbying activities regarding legislation, rules, regulations, etc.

Query 304 - Documents that could be withheld from production on grounds of privilege, attorney work-product, or other applicable protection.
\item The document collection is derived from about 1.3 million emails captured from Enron by the Federal Energy Regulatory Commission (FERC) during its investigation of Enron's bankruptcy. The emails contain parent emails and attachments in various formats.

\item The relevance is binary - either relevant (1) or not relevant (0) for each document/message assessed.

\item We annotate instructions like this "Given a request for production in civil litigation, retrieve all documents or communications from the database that are responsive to this request while minimizing the number of unresponsive documents that are retrieved. The database consists of email messages captured by the Federal Energy Regulatory Commission (FERC) from Enron, in the course of its investigation of Enron."

\item The following is an example:
[A table]
\end{itemize}
\subsubsection{TREC Legal Track 2011}
The same as \ref{legal10}
\subsubsection{TREC NeuCLIR track 2022} \label{neu22}
This track studies cross-language information retrieval (CLIR) and multi-lingual information retrieval (MLIR) tasks. It uses English queries to retrieve news documents in Chinese, Persian, and Russian, as well as Chinese technical documents like dissertation abstracts. Notably, all documents in the collection are News documents that have been machine-translated into English. 
\begin{itemize}
\item The queries are human-created, containing an English title, description and narrative to simulate real information needs.

\item The documents include news articles in Chinese, Persian and Russian, as well as Chinese technical documents like dissertation abstracts covering fields such as chemistry, physics, computer science and more. The news articles are from newswire sources, while the technical documents are from a Chinese scientific literature database. Document lengths vary from a few sentences to a few hundred words.

\item The basis for judging relevance is whether a document contains core information related to the query topic. The relevance is divided into 4 levels:
\begin{itemize}
    \item Highly relevant(3): document is fully relevant to the topic (i.e., it contains facts that would be included in the lead paragraph of a report on the topic)
    \item No documents(2): there are no documents with relevant judgment
    \item Somewhat relevant(1): document is somewhat relevant to the topic (i.e., it contains facts that would be included elsewhere in a report on the topic)
    \item Nor relevant(0): document is not relevant to the topic (i.e., it does not contain information that would be included in a report written about the topic)
\end{itemize}

\item Instruction is related to the query, and each query has different instructions.

\item The following is an example:
[A table]
\end{itemize}
\subsubsection{TREC NeuCLIR track 2023}
The TREC NeuCLIR track 2023 has two tasks: 1) Cross-language and multilingual news retrieval across three languages, which is the same as \ref{neu22} and 2) A pilot task for retrieving Chinese technical/academic content in a cross-language setting using English queries.

\paragraph{Technical Documents Pilot Task}
The pilot technical document task examines feasibility over diverse technical domains by retrieving Chinese academic abstracts using English queries, with optional monolingual runs using translated Chinese queries.

\begin{itemize}
\item Queries in this task are created by graduate students across various technical disciplines, with the topics focused on their specific research areas. 

\item Documents in this task is a large set of nearly 400,000 Chinese academic paper and thesis abstracts covering a wide range of technical disciplines like engineering, science, medicine, etc. published in the 2010-2020 time period. These technical abstracts formed the target corpus that systems had to search over using the provided English topics.

All documents have been machine-translated into English. 
\item The relevance judgment is the same as \ref{neu22}

\item Instruction is related to the query, and each query has different instructions.

\item The following is an example:
[A table]
\end{itemize}
\subsubsection{TREC Product Search Track 2023} \label{ps23}
This track studies the product search retrieval task. It uses synthetically generated queries to retrieve product descriptions and metadata documents from Amazon's online product catalog.
\begin{itemize}
\item The queries are generated in two ways: 1) 500 queries are generated using GPT-4 based on prompts, and 2) substrings are extracted from product titles and descriptions as queries. In total, 998 evaluation queries are generated.

\item The documents are product descriptions and metadata, including reviews, dimensions, colors, and other attributes, as well as 1-10 64x64 thumbnail images crawled from Amazon's online catalog(not used in our setting). The data is sourced from the ESCI Product Re-ranking dataset, but only English products are retained and enriched with additional metadata from Amazon.

\item The basis for judging relevance levels is the degree of match between the product and the query. Relevance is divided into 4 levels:
\begin{itemize}
    \item Perfectly relevant(3): The product is exactly what the user wants.
    \item Highly relevant(2): The product could match the user query, but it may be a substitute for the original query intent. It may have a slightly different style, brand, or type, but a user would be satisfied if they received this product.
    \item Related(1): The product seems related to the query but not the item the user seeks. Products in this category could complement the user’s intended product.
    \item Irrelevant(0): The product has nothing to do with the query.
\end{itemize}

\item We annotate instructions like this "Given a search query, retrieve products that are relevant to the query."

\item The following is an example:
[A table]
\end{itemize}
\subsubsection{TREC Product Search Track 2024}
The same as \ref{ps23}
\subsubsection{TREC Tip-of-the-Tongue Track 2023} \label{tot23}
This track studied the tip-of-the-tongue (ToT) known-item retrieval task, using queries sampled from an existing ToT dataset to retrieve a corpus of Wikipedia pages associated with the "audiovisual works" category.
\begin{itemize}
\item The queries originated from the "I Remember This Movie..." forum, where users post ToT requests for movies. These queries tend to be verbose and include complex phenomena such as information about the movie itself (semantic memories), the context in which the searcher last encountered the movie (episodic memories), mentions of uncertainty, exclusion criteria, relative comparisons, and false memories.

\item The document corpus is constructed from Wikipedia and contained pages associated with the "audiovisual works" category. This corpus included the correct answer for all training, development, and test queries. The documents consisted of multiple fields, including the page source code, parsed infoboxes, etc.

\item The relevance is essentially a binary judgment - either a document is the one correct answer for that query topic (1), or it is not relevant(0). 

\item We annotate instructions like this "You are an expert in movies, assisting someone in recalling the name of a movie that's on the tip of their tongue. For the given tip-of-the-tongue information requests, retrieve Wikipedia pages of potential movie titles that match the description provided."

\item The following is an example:
[A table]
\end{itemize}
\subsubsection{TREC Tip-of-the-Tongue Track 2024}
The same as \ref{tot23}

\subsection{SIGIR}\label{SIGIR}
\subsubsection{ACORDAR}
The paper studies the task of ad hoc content-based dataset retrieval. Keyword queries are used to retrieve datasets, where the target documents are the metadata and data content of the datasets. 

\begin{itemize}
    \item The queries come in two forms: synthetic and TREC queries. 
    Synthetic queries are created by human annotators by summarizing the content of a dataset they browsed, aiming to match the dataset's content. 
    TREC queries are general topic queries from the TREC test collections.
    \item The documents are datasets containing metadata (e.g. title, description, author) and data content (RDF triples). 
    These datasets are from 543 open data portals across multiple domains, in the RDF data format. 
    The datasets vary greatly in data size and schema size.
    \item Relevance is judged based on whether the information contained in a dataset would be used when writing a report or developing an application on the topic of the query. 
    The relevance is divided into 3 levels:
    \begin{itemize}
        \item Irrelevant(0): the dataset is completely unrelated to the query topic, and none of its information would be used.
        \item Partially relevant(1): the dataset has some content related to the query topic, and some of its information may be used, but not all.
        \item Highly relevant(2): the dataset is highly related to the query topic, and much of its contained information would be heavily used. It can largely satisfy the information needs of the query.
    \end{itemize}
    \item We annotate instructions like this "Given a question, identify and retrieve datasets where the keywords in the query may be found in either the metadata or the actual data of the dataset."
\end{itemize}

\subsubsection{ChroniclingAmericaQA}
This paper studies the open-domain question-answering task, using natural language questions as queries to retrieve relevant answers from the Chronicling America collection of historical American newspaper pages.

\begin{itemize}
    \item The queries used are natural language questions, such as "How many subscribers did Jackson lose on Saturday?". 
    These questions are automatically generated based on the content of the newspaper articles.
    \item The document collection used for retrieval is the Chronicling America collection of historical American newspapers. 
    It is a large digital archive containing over 21 million pages of newspapers published between 1756 and 1963, covering information ranging from major historical events to everyday life details. 
    The documents are available in both scanned image and OCR text formats.
    \item The ChroniclingAmericaQA dataset uses a binary relevance classification:
    \begin{itemize}
        \item Relevant(1): The answer comes from the given historical newspaper document collection and is semantically relevant to the question, providing an answer to the query.
        \item Not Relevant(0): The answer does not come from the given document collection, or even if it does, it is semantically unrelated to the question and cannot answer the query.
    \end{itemize}
    \item We annotate instructions like this "Given a question, retrieve newspaper pages that contain the answer to the question from the American historical newspaper dataset Chronicling America."
\end{itemize}

\subsubsection{CPCD}
This paper studies a new retrieval task called Conversational Item Set Curation. In this task, a user engages in a conversation with a system to curate a small set of items (e.g. a music playlist) from a larger collection. The system needs to retrieve relevant items (e.g. songs) based on the conversation history and recommend them to the user.

\begin{itemize}
    \item The query is formed from the conversation history, comprising all previous user utterances. 
    For example, the user may first state a theme ("Create a rock playlist for a long drive"), and then provide additional details and preferences in subsequent turns ("Do you have anything from old Stevie Wonder?").
    \item The documents are the items in the collection to be retrieved, which in this work are songs. 
    Each song is represented as a text document in the format "<title> by <artist> from <album>". The song data comes from expert-curated playlist descriptions.
    \item Relevance is judged based on the preferences expressed by the user during the conversation. 
    A song is considered relevant if it matches the theme, genre, artist, etc. mentioned by the user. 
    The relevance is divided into 4 levels:
    \begin{itemize}
        \item Highly relevant(3): Matches all preferences expressed by the user
        \item Relevant(2): Matches most of the preferences expressed
        \item Partially relevant(1): Matches some of the preferences expressed
        \item Not relevant(0): Does not match any of the expressed preferences
    \end{itemize}
    \item We annotate instructions like this "The query is a dialogue history in which the user seeks music recommendations. In each turn, the system recommends some music, and the user provides feedback indicating whether they like or dislike the recommendations. Based on the user's preferences and requests, retrieve music that the user is likely to enjoy as the recommendation response."
\end{itemize}

\subsubsection{Monant}
This paper studies the task of detecting medical misinformation. Specifically, given a fact-checked medical claim, it aims to retrieve news articles or blog posts that contain that claim.

\begin{itemize}
    \item The queries used are fact-checked medical claims, e.g. "Omega-3 fatty acids decrease triglycerides".
    \item The documents being retrieved are medical news articles and blog posts. These articles come from multiple reliable and unreliable website sources and include text content, images, videos, etc. The data is collected from the web using web crawlers.
    \item The basis for relevance levels is whether the article contains the given claim, and what stance the article takes towards that claim (supporting, contradicting, or neutral). The relevance levels are:
    \begin{itemize}
        \item Present(1): The article contains a sentence or paragraph that is literally or semantically similar to the claim
        \item Not present(2): The article does not contain the claim
        \item Supporting(3) The article supports the claim
        \item Contradicting(4) The article contradicts the claim
        \item Neutral(5) The article has a neutral stance toward the claim
    \end{itemize}
    \item We annotate instructions like this "Given a medical claim, retrieve articles that either support or contradict the claim."
\end{itemize}

\subsubsection{NTCIR}
The paper introduces a new test collection for ad-hoc dataset retrieval. The task is to retrieve relevant datasets from open government data portals (Data.gov and e-Stat) given a query derived from real information needs.

\begin{itemize}
    \item The queries are keyword queries transformed from real information needs, aiming to capture users' actual search intents.
    \item The documents being retrieved are datasets from the government's open data portals, where each dataset contains metadata and one or more data files, mainly from Data.gov (US) and e-Stat (Japan) covering various domains.
    \item Relevance judgments are based on how useful a dataset is for satisfying the information need behind the query, with 3 grades:
    \begin{itemize}
        \item Irrelevant(0): The dataset is completely irrelevant to the query.
        \item Partially relevant(1): The dataset contains some relevant content but cannot fully satisfy the need.
        \item Highly relevant(2) The dataset can well satisfy the information need of the query.
    \end{itemize}
    \item We annotate instructions like this "Given a search query, retrieve relevant datasets from Data.gov and e-Stat that contain the requested information."
\end{itemize}

\subsubsection{PointRec}
This paper studies a point-of-interest (POI) recommendation task driven by natural language descriptions. User queries are natural language descriptions of their travel needs and preferences, which are used to retrieve from a document collection of 695,000 POI entries.

\begin{itemize}
    \item The queries are in the form of natural language descriptions, specifying the user's travel destination, preferred categories (e.g. restaurants, nightlife), travel group, specific requirements or constraints on the POIs, etc. For example, "I want to find a not-too-noisy restaurant with good service near London to take my 80-year-old dad for a meal."
    \item The document collection contains 695,000 POI entries collected from Yelp's online directory, spanning over 2,000 cities across 23 countries. Each POI entry includes basic information like name, address, categories, rating, and review count, and is linked to the GeoNames geographical knowledge base for location data. Relevant text snippets are also extracted from web search results as descriptions. So this is a cross-domain document collection containing both structured data and unstructured text.
    \item The relevance judgments are primarily based on whether the POI satisfies the destination, category, travel group, and specific requirements or constraints described in the query. The relevance levels are:
    \begin{itemize}
        \item Highly relevant(3): The POI perfectly matches the location, category, and all constraints specified in the query
        \item Relevant(2): The location and category match and the requester would likely be interested
        \item Somewhat relevant(1): The location matches, and the requester could possibly be interested  
        \item Not relevant(0): The POI does not satisfy any of the above conditions
    \end{itemize}
    \item We annotate instructions like this "Given a user's request, recommend a point of interest (POI) that best matches the user's intent. Use the following metadata for reference:{'Group': xx, 'Main Category': xx, 'Sub Categories': [xx, ...], ...}"
\end{itemize}
\subsubsection{ProCIS}
The paper studies the task of proactive retrieval, where the system proactively retrieves and recommends documents relevant to an ongoing multi-party conversation, without the user explicitly providing a query. The query is the entire conversation history, and the documents are from Wikipedia articles.

The paper studies two different tasks:

Turn-level Proactive Retrieval: In this task, the system needs to decide whether to retrieve documents at each turn of the conversation. If it decides to retrieve, it needs to return a ranked list of documents as contextual suggestions for that turn.

Dialog-level Reactive Retrieval: In this task, the system needs to retrieve relevant documents based on the entire conversation history after the conversation is finished, as contextual suggestions for the whole dialogue.

\begin{itemize}
    \item The query is the full context history of an ongoing multi-party human-machine conversation. The system needs to understand the conversation context and proactively retrieve documents relevant to the conversation at opportune moments as suggestions.
    \item The documents are articles from Wikipedia, covering a wide range of topics such as politics, religion, sports, finance, science, etc. These documents can provide useful background information, context, or supplementary knowledge for the ongoing conversation. The data source is Reddit conversation threads, which are cleaned and augmented by linking to Wikipedia articles.
    \item The basis for relevance levels is the degree to which the document is associated with the conversation, i.e., how much useful background information and context the document provides for the conversation.
    There are 3 relevance levels:
    \begin{itemize}
        \item Provides Useful Context (2): The document is directly related to the conversation, providing substantial useful background information or supplementary knowledge that enhances the understanding of the conversation.
        \item Partially Relevant (1): The document is somewhat related to the conversation. It provides some context or additional information but is not directly tied to the main topic of the conversation.
        \item Irrelevant (0): The document is completely unrelated to the conversation and does not provide any useful context or additional information.
    \end{itemize}
    \item We annotate instructions like this "Given a multi-party human conversation (such as a Reddit post and its comments), retrieve relevant documents from Wikipedia to provide contextual information. The criteria for relevance are as follows: ..."
\end{itemize}

\subsubsection{QuanTemp}
This paper studies the retrieval task for numerical claims for fact-checking. It uses the original claims and questions generated from claim decomposition as queries to retrieve relevant evidence documents from the web.

\begin{itemize}
    \item The queries include the original numerical claims as well as a series of questions decomposed from the claims using methods like ClaimDecomp and Program-FC. For example, for the claim "The ICE spends 4 times the amount to detain a person for a year than on a student in public school", the decomposed questions could include "How much does ICE spend to detain a person for a year?", "How much is spent on a student in public school?" etc.
    \item The documents are relevant to web page snippets retrieved from the internet, covering domains like Wikipedia, government websites, statistics websites, etc. These snippets do not include any content from fact-checking websites to prevent the model from learning shortcuts. A total of 423,320 such evidence snippets are collected.
    \item The relevance levels are classified based on the usefulness of the evidence snippets in verifying the original claim.
    The relevance levels are as follows:
    \begin{itemize}
        \item Highly relevant(3): Evidence snippet directly supports or refutes the claim
        \item Partially relevant(2): Evidence snippet contains information helpful in verifying parts of the claim
        \item Not relevant(1): The evidence snippet is not related to the claim
        \item Contradictory(0): Evidence snippet contradicts the claim
    \end{itemize}
    \item We annotate instructions like this "Given a numerical claim, retrieve documents that can verify the claim."
\end{itemize}

% \subsubsection{RecMeApp}
% This paper studies the task of mobile app recommendation. It does not use queries to retrieve documents. Instead, it constructs a large-scale dataset called MobileRec containing user interactions with mobile apps, which is used to train and evaluate recommendation models.

% \begin{itemize}
%     \item No query
%     \item The document refers to the MobileRec dataset, which contains 19.3 million user reviews and ratings for mobile apps from the Google Play Store, covering 10,173 distinct apps across 48 categories. Each record includes rich information such as user ID, app details, review text, rating score, and timestamp. It is a large-scale sequential user-app interaction dataset.
%     \item The relevance levels are as follows:
%     \begin{itemize}
%         \item Highly relevant(3): The recommendation system performs excellently on the evaluation metrics for this dataset.
%         \item Moderately relevant(2): The recommendation system has average performance on the evaluation metrics for this dataset. 
%         \item Slightly relevant(1): The recommendation system performs poorly on the evaluation metrics for this dataset.
%         \item Not relevant(0): The recommendation system completely fails to work well on this dataset.
%     \end{itemize}
% \end{itemize}

\subsubsection{WebTableSearch}
This paper studies the task of web table retrieval. It uses keyword queries to retrieve a set of relevant web tables.

\begin{itemize}
    \item The query is a set of keywords describing the user's information need, e.g. "Fast cars".
    \item The documents are HTML tables extracted from the Common Crawl web corpus. These tables are from 61,086 different domain names, covering a broad range of topics. In addition to the table itself, each table has associated context fields such as page title, text before/after the table, and entities linked to DBpedia.
    \item The relevance levels are judged based on how relevant the query is to the table and its context fields (e.g. page title, surrounding text).
    There are 3 relevance levels:
    \begin{itemize}
        \item Not relevant(0): This field is not relevant to the query.
        \item Relevant (1): This field provides relevant information about the query.
        \item Highly relevant (2): This field provides ideal information about the query.
    \end{itemize}
    \item We annotate instructions like this "Given a question, retrieve relevant table to answer the question."
\end{itemize}
